# Supplementary material for: Inference on Individual Treatment Effects in Nonseparable Triangular Models
Source: arXiv:2107.05559 ancillary file (2023-02-15)
Supplement: Supplementary file 1 [file Supplement_V2.pdf]

# Supplement to “Inference on Individual Treatment Effects in Nonseparable Triangular Models”

Jun Ma\*

Vadim Marmer<sup>†</sup>

Zhengfei Yu<sup>‡</sup>

## Abstract

The supplement collects all omitted proofs from the main text and provides some additional Monte Carlo simulation results.

## S1 Proofs of Lemmas 1, 2 and 3

**Proof of Lemma 1.** Let  $\Pi_{dzz}(y) := \Pr[Y \leq y, D = d, Z = z, X = x]$  and  $\hat{\Pi}_{dzz}(y) := n^{-1} \sum_{i=1}^n \mathcal{D}_{dzz}(W_i; y)$ , where  $\mathcal{D}_{dzz}(W_i; y) := \mathbb{1}(Y_i \leq y, D_i = d, Z_i = z, X_i = x)$ . Let  $\hat{p}_{zx} := n^{-1} \sum_{i=1}^n \mathbb{1}(Z_i = z, X_i = x)$ . Let  $I_{dx} := \mathcal{S}_{Y_{dx}|X=x}$ . It follows from Kosorok (2007, Lemmas 9.7(iv) and 9.8) that the class  $\mathfrak{D} := \{\mathcal{D}_{dzz}(\cdot; y) : y \in I_{dx}\}$  is VC-subgraph with VC index being at most 2. Then it follows from Giné and Nickl (2016, Theorem 3.6.9) that  $\mathfrak{D}$  is VC-type with respect to the constant envelope  $F_{\mathfrak{D}} = 1$ . It follows from Talagrand’s inequality (Chernozhukov et al., 2016, Lemma 6.3, with  $\mathcal{F} = \mathfrak{D}$ ,  $\sigma = b = F_{\mathfrak{D}} = 1$  and  $t = \log(n)$ ) that  $\|\mathbb{G}_n^W\|_{\mathfrak{D}} = O_p^*(\sqrt{\log(n)})$ . Note that  $\|\hat{\Pi}_{dzz} - \Pi_{dzz}\|_{I_{dx}} = n^{-1/2} \|\mathbb{G}_n^W\|_{\mathfrak{D}}$  and therefore,  $\|\hat{\Pi}_{dzz} - \Pi_{dzz}\|_{I_{dx}} = O_p^*(\sqrt{\log(n)/n})$ . It follows from similar arguments that  $\|\hat{Q}_{dx} - Q_{dx}\|_{\mathcal{B}} = O_p^*(\sqrt{\log(n)/n})$  for any compact set  $\mathcal{B} \subseteq \mathbb{R}^2$ . Then it is straightforward to strengthen FVX’s uniform consistency result for  $\|\hat{\phi}_{dx} - \phi_{dx}\|_{I_{d'x}}$ . By arguments used in the proof of Angrist et al. (2006, Theorem 3),  $\forall \delta > 0$ , there exists a positive constant  $C$  such that,  $\Pr\left[\|\hat{\phi}_{dx} - \phi_{dx}\|_{I_{d'x}} \leq \delta\right] \geq 1 - Cn^{-1}$ , when  $n$  is sufficiently large.

It is shown in the proof of Theorem 1 of FVX that

$$\left(\frac{\hat{\Pi}_{d0x}(\hat{\phi}_{dx}(y))}{\hat{p}_{0x}} - \frac{\hat{\Pi}_{d1x}(\hat{\phi}_{dx}(y))}{\hat{p}_{1x}}\right) + \left(\frac{\hat{\Pi}_{d'0x}(y)}{\hat{p}_{0x}} - \frac{\hat{\Pi}_{d'1x}(y)}{\hat{p}_{1x}}\right) = \varepsilon_n, \quad (\text{S1})$$

with a bounded error term that satisfies  $|\varepsilon_n| \leq n^{-1}$  and therefore  $\varepsilon_n = O_p^*(n^{-1})$ . Note that  $\phi_{dx}(y)$  satisfies

$$\left(\frac{\Pi_{d0x}(\phi_{dx}(y))}{p_{0x}} - \frac{\Pi_{d1x}(\phi_{dx}(y))}{p_{1x}}\right) + \left(\frac{\Pi_{d'0x}(y)}{p_{0x}} - \frac{\Pi_{d'1x}(y)}{p_{1x}}\right) = 0. \quad (\text{S2})$$

Note that  $\zeta_{dx}(y) = \Pi'_{d1x}(y)/p_{1x} - \Pi'_{d0x}(y)/p_{0x}$ . It follows from Hoeffding’s inequality that  $\hat{p}_{zx} - p_{zx} = O_p^*(\sqrt{\log(n)/n})$  and it is easy to check that this also implies  $\hat{p}_{zx}^{-1} - p_{zx}^{-1} = O_p^*(\sqrt{\log(n)/n})$ . Note that by

---

This version: July 7, 2021.

\*School of Economics, Renmin University of China, P.R. China

<sup>†</sup>Vancouver School of Economics, University of British Columbia, Canada

<sup>‡</sup>Faculty of Humanities and Social Sciences, University of Tsukuba, Japan

construction,  $\widehat{\phi}_{dx}(y) \in I_{dx}$ . Then it follows from these results, (S1), (S2),  $\|\widehat{\Pi}_{dzz} - \Pi_{dzz}\|_{I_{dx}} = O_p^*\left(\sqrt{\log(n)/n}\right)$  and also Assumption 4(c) that  $\|\widehat{\phi}_{dx} - \phi_{dx}\|_{I_{d'x}} = O_p^*\left(\sqrt{\log(n)/n}\right)$ , i.e., for some constant  $C_1, C_2$ , when  $n$  is sufficiently large,

$$\Pr \left[ \|\widehat{\phi}_{dx} - \phi_{dx}\|_{I_{d'x}} \leq C_1 \sqrt{\frac{\log(n)}{n}} \right] > 1 - C_2 n^{-1}. \quad (\text{S3})$$

And then we also have  $\|\widehat{\Pi}_{dzz} \circ \widehat{\phi}_{dx} - \Pi_{dzz} \circ \phi_{dx}\|_{I_{d'x}} = O_p^*\left(\sqrt{\log(n)/n}\right)$ . By using this result, (S1), (S2),  $\|\widehat{\Pi}_{dzz} - \Pi_{dzz}\|_{I_{dx}} = O_p^*\left(\sqrt{\log(n)/n}\right)$  and the equality

$$\frac{a}{b} = \frac{a}{c} - \frac{a(b-c)}{c^2} + \frac{a(b-c)^2}{bc^2}, \quad (\text{S4})$$

we have

$$\begin{aligned} O_p^*\left(\frac{\log(n)}{n}\right) &= \left( \frac{\widehat{\Pi}_{d0x}(\widehat{\phi}_{dx}(y))}{p_{0x}} - \frac{\Pi_{d0x}(\phi_{dx}(y))}{p_{0x}} \right) - \left( \frac{\widehat{\Pi}_{d1x}(\widehat{\phi}_{dx}(y))}{p_{1x}} - \frac{\Pi_{d1x}(\phi_{dx}(y))}{p_{1x}} \right) \\ &+ \left( \frac{\widehat{\Pi}_{d'0x}(y)}{p_{0x}} - \frac{\Pi_{d'0x}(y)}{p_{0x}} \right) - \left( \frac{\widehat{\Pi}_{d'1x}(y)}{p_{1x}} - \frac{\Pi_{d'1x}(y)}{p_{1x}} \right) - \frac{\Pi_{d0x}(\phi_{dx}(y))}{p_{0x}^2} (\widehat{p}_{0x} - p_{0x}) + \frac{\Pi_{d1x}(\phi_{dx}(y))}{p_{1x}^2} (\widehat{p}_{1x} - p_{1x}) \\ &\quad - \frac{\Pi_{d'0x}(y)}{p_{0x}^2} (\widehat{p}_{0x} - p_{0x}) + \frac{\Pi_{d'1x}(y)}{p_{1x}^2} (\widehat{p}_{1x} - p_{1x}). \end{aligned} \quad (\text{S5})$$

Decompose  $\widehat{\Pi}_{dzz}(\widehat{\phi}_{dx}(y)) - \Pi_{dzz}(\phi_{dx}(y))$  into the sum of  $\widehat{\Pi}_{dzz}(\widehat{\phi}_{dx}(y)) - \Pi_{dzz}(\widehat{\phi}_{dx}(y))$  and  $\Pi_{dzz}(\widehat{\phi}_{dx}(y)) - \Pi_{dzz}(\phi_{dx}(y))$ . We will later show that

$$\widehat{\Pi}_{dzz}(\widehat{\phi}_{dx}(y)) - \Pi_{dzz}(\widehat{\phi}_{dx}(y)) = \widehat{\Pi}_{dzz}(\phi_{dx}(y)) - \Pi_{dzz}(\phi_{dx}(y)) + O_p^*\left(\left(\frac{\log(n)}{n}\right)^{3/4}\right), \quad (\text{S6})$$

uniformly in  $y \in I_{d'x}$ . By a second-order Taylor expansion,

$$\begin{aligned} &\left( \frac{\Pi_{d1x}(\widehat{\phi}_{dx}(y))}{p_{1x}} - \frac{\Pi_{d0x}(\widehat{\phi}_{dx}(y))}{p_{0x}} \right) - \left( \frac{\Pi_{d1x}(\phi_{dx}(y))}{p_{1x}} - \frac{\Pi_{d0x}(\phi_{dx}(y))}{p_{0x}} \right) = \\ &\quad \zeta_{dx}(\phi_{dx}(y)) (\widehat{\phi}_{dx}(y) - \phi_{dx}(y)) + O_p^*\left(\frac{\log(n)}{n}\right), \end{aligned} \quad (\text{S7})$$

uniformly in  $y \in I_{d'x}$ . Note that if  $X = x$ ,

$$\begin{aligned} \mathbb{1}(Y \leq \phi_{dx}(y), D = d) + \mathbb{1}(Y \leq y, D = d') &= \mathbb{1}(g(d, x, \epsilon) \leq \phi_{dx}(y), D = d) + \mathbb{1}(g(d', x, \epsilon) \leq y, D = d') \\ &= \mathbb{1}(g(d', x, \epsilon) \leq y). \end{aligned} \quad (\text{S8})$$

Since  $Z$  is conditionally independent of  $\epsilon$  given  $X$ ,  $\forall z \in \{0, 1\}$ ,

$$\begin{aligned} R_{d'x}(y) &= \mathbb{E}[\mathbb{1}(Y \leq \phi_{dx}(y), D = d) + \mathbb{1}(Y \leq y, D = d') | X = x, Z = z] \\ &= \frac{\Pi_{dzz}(\phi_{dx}(y))}{p_{zx}} + \frac{\Pi_{d'zx}(y)}{p_{zx}} \\ &= F_{d'x|x}(y), \end{aligned} \quad (\text{S9})$$

where  $F_{d'x|x}(y) := \Pr[Y_{d'x} \leq y | X = x]$ . Combining (S5), (S6) and (S7) and then using (S9), we have

$$\begin{aligned} \zeta_{dx}(\phi_{dx}(y)) \left( \widehat{\phi}_{dx}(y) - \phi_{dx}(y) \right) = \\ \frac{\widehat{\Pi}_{d0x}(\phi_{dx}(y))}{p_{0x}} - \frac{\widehat{\Pi}_{d1x}(\phi_{dx}(y))}{p_{1x}} + \frac{\widehat{\Pi}_{d'0x}(y)}{p_{0x}} - \frac{\widehat{\Pi}_{d'1x}(y)}{p_{1x}} - R_{d'x}(y) \frac{\widehat{p}_{0x}}{p_{0x}} + R_{d'x}(y) \frac{\widehat{p}_{1x}}{p_{1x}} + O_p^* \left( \left( \frac{\log(n)}{n} \right)^{3/4} \right) = \\ \frac{1}{n} \sum_{i=1}^n (\mathbb{1}(Y_i \leq \phi_{dx}(y), D_i = d) + \mathbb{1}(Y_i \leq y, D_i = d') - R_{d'x}(y)) \left( \frac{\mathbb{1}(Z_i = 0, X_i = x)}{p_{0x}} - \frac{\mathbb{1}(Z_i = 1, X_i = x)}{p_{1x}} \right) \\ + O_p^* \left( \left( \frac{\log(n)}{n} \right)^{3/4} \right). \end{aligned}$$

The conclusion follows from this result. It remains to show (S6).

Denote  $\widehat{\Lambda}_{dzz}(y, y') := \widehat{\Pi}_{dzz}(y) - \widehat{\Pi}_{dzz}(y')$  and  $\Lambda_{dzz}(y, y') := \Pi_{dzz}(y) - \Pi_{dzz}(y')$ . In view of (S3), denote  $\bar{\xi} := C_1 \sqrt{\log(n)}/n$ . For  $\xi > 0$ , denote  $\mathcal{P}_{dzz}^+(W_i; y, \xi) := \mathbb{1}(\phi_{dx}(y) < Y_i \leq \phi_{dx}(y) + \xi, D_i = d, Z_i = z, X_i = x)$  and  $\mathcal{P}_{dzz}^-(W_i; y, \xi) := \mathbb{1}(\phi_{dx}(y) - \xi < Y_i \leq \phi_{dx}(y), D_i = d, Z_i = z, X_i = x)$ . By Kosorok (2007, Lemmas 9.7(iv) and 9.8), the function class  $\mathfrak{P}^+ := \{\mathcal{P}_{dzz}^+(\cdot; y, \xi) : y \in I_{d'x}, \xi \in (0, \bar{\xi}]\}$  is VC-subgraph with VC index being at most 3,  $\forall n$ , and by Giné and Nickl (2016, Theorem 3.6.9),  $\mathfrak{P}^+$  is uniformly VC-type with respect to the constant envelope  $F_{\mathfrak{P}^+} = 1$ .  $\mathfrak{P}^-$  is defined similarly. Then,

$$\begin{aligned} \sup_{y \in I_{d'x}} \left| \left\{ \widehat{\Pi}_{dzz}(\widehat{\phi}_{dx}(y)) - \widehat{\Pi}_{dzz}(\phi_{dx}(y)) \right\} - \left\{ \Pi_{dzz}(\widehat{\phi}_{dx}(y)) - \Pi_{dzz}(\phi_{dx}(y)) \right\} \right| \leq \\ \sup_{(y, \xi) \in I_{d'x} \times [-\bar{\xi}, \bar{\xi}]} \left| \widehat{\Lambda}_{dzz}(\phi_{dx}(y) + \xi, \phi_{dx}(y)) - \Lambda_{dzz}(\phi_{dx}(y) + \xi, \phi_{dx}(y)) \right| \leq \\ \|\mathbb{P}_n^W - \mathbb{P}^W\|_{\mathfrak{P}^+} + \|\mathbb{P}_n^W - \mathbb{P}^W\|_{\mathfrak{P}^-}, \quad (\text{S10}) \end{aligned}$$

where the first inequality holds with probability at least  $1 - C_2 n^{-1}$ . We have

$$\begin{aligned} \mathbb{E} \left[ \mathcal{P}_{dzz}^+(W; y, \xi)^2 \right] &= \mathbb{E} \left[ \left( \mathbb{1}(Y \leq \phi_{dx}(y) + \xi) - \mathbb{1}(Y \leq \phi_{dx}(y)) \right)^2 \mathbb{1}(D = d, Z = z, X = x) \right] \\ &= \left( \int_{\phi_{dx}(y)}^{\phi_{dx}(y) + \xi} f_{Y|DZX}(y' | d, z, x) dy' \right) \Pr[D = d, Z = z, X = x] \end{aligned}$$

and since  $f_{Y|DZX}$  is bounded under Assumptions 1 and 4,

$$\sigma_{\mathfrak{P}^+}^2 := \sup_{f \in \mathfrak{P}^+} \mathbb{P}^W f^2 = \sup_{(y, \xi) \in I_{d'x} \times (0, \bar{\xi}]} \mathbb{E} \left[ \mathcal{P}_{d0x}^+(W; y, \xi)^2 \right] = O \left( \left( \frac{\log(n)}{n} \right)^{1/2} \right).$$

By Talagrand's inequality ( $\mathcal{F} = \mathfrak{P}^+$ ,  $b = F_{\mathfrak{P}^+} = 1$ ,  $\sigma = \sigma_{\mathfrak{P}^+} \vee n^{-1/4} b$ ,  $t = \log(n)$ ),  $\|\mathbb{G}_n^W\|_{\mathfrak{P}^+} = O_p^* \left( \log(n)^{3/4} / n^{1/4} \right)$ . A similar result holds for  $\|\mathbb{G}_n^W\|_{\mathfrak{P}^-}$ . (S6) follows from these results and (S10).  $\blacksquare$

**Proof of Lemma 2.** By Taylor expansion,

$$\begin{aligned} \widehat{f}_{\Delta X}(v, x) - \widetilde{f}_{\Delta X}(v, x) &= \frac{1}{n} \sum_{i=1}^n \frac{1}{h^2} K' \left( \frac{\Delta_i - v}{h} \right) (\widehat{\Delta}_i - \Delta_i) \mathbb{1}(X_i = x) \\ &\quad + \frac{1}{2} \frac{1}{n} \sum_{i=1}^n \frac{1}{h^3} K'' \left( \frac{\Delta_i - v}{h} \right) (\widehat{\Delta}_i - \Delta_i)^2 \mathbb{1}(X_i = x), \quad (\text{S11}) \end{aligned}$$

where  $\dot{\Delta}_i$  denotes the mean value that lies between  $\hat{\Delta}_i$  and  $\Delta_i$ . It is easy to see from the proof of Lemma 1 that (S3) also holds for  $\hat{\phi}_{dx}^{-i}(y)$  uniformly in  $i = 1, \dots, n$ . Therefore,

$$\bar{\Delta} := \max_{i=1, \dots, n} |\hat{\Delta}_i - \Delta_i| \mathbb{1}(X_i = x) = O_p^* \left( \sqrt{\frac{\log(n)}{n}} \right). \quad (\text{S12})$$

In view of  $\Pr \left[ \bar{\Delta} > C_1 \sqrt{\log(n)/n} \right] \leq C_2 n^{-1}$ , with probability at least  $1 - C_2 n^{-1}$ ,  $\bar{\Delta} \leq h$ , when  $n$  is sufficiently large. And therefore, by the triangle inequality, with probability at least  $1 - C_2 n^{-1}$ ,

$$\sup_{v \in I_x} \left| \frac{1}{n} \sum_{i=1}^n \frac{1}{h^3} K'' \left( \frac{\dot{\Delta}_i - v}{h} \right) (\hat{\Delta}_i - \Delta_i)^2 \mathbb{1}(X_i = x) \right| \lesssim \left\{ \sup_{v \in I_x} \frac{1}{n} \sum_{i=1}^n h^{-3} \mathbb{1}(|\Delta_i - v| \leq 2h) \mathbb{1}(X_i = x) \right\} \bar{\Delta}^2, \quad (\text{S13})$$

when  $n$  is sufficiently large. Let  $\mathcal{I}_x(U_i; v) := h^{-1} \mathbb{1}(|\Delta_x(\epsilon_i) - v| \leq 2h) \mathbb{1}(X_i = x)$ . It follows from Kosorok (2007, Lemmas 9.7(iv), 9.8 and 9.9(vii,viii)) that  $\mathfrak{I} := \{\mathcal{I}_x(\cdot; v) : v \in I_x\}$  is VC-subgraph with VC index being at most 3,  $\forall h$ , and has a constant envelope  $F_{\mathfrak{I}} = h^{-1}$ . Therefore, by Giné and Nickl (2016, Theorem 3.6.9),  $\mathfrak{I}$  is uniformly VC-type with respect to the constant envelope  $F_{\mathfrak{I}}$ . It is easy to check that  $\|\mathbb{P}^U\|_{\mathfrak{I}} = O(1)$  and  $\sigma_{\mathfrak{I}}^2 := \sup_{f \in \mathfrak{I}} \mathbb{P}^U f^2 = O(h^{-1})$ . By Talagrand's inequality ( $\mathcal{F} = \mathfrak{I}$ ,  $b = F_{\mathfrak{I}}$ ,  $\sigma = \sigma_{\mathfrak{I}} \vee n^{-1/2}b$ ,  $t = \log(n)$ ),  $\|\mathbb{G}_n^U\|_{\mathfrak{I}} = O_p^* \left( \sqrt{\log(n)/h} \right)$  and therefore,

$$\sup_{v \in I_x} \frac{1}{n} \sum_{i=1}^n h^{-1} \mathbb{1}(|\Delta_i - v| \leq 2h) \mathbb{1}(X_i = x) = \|\mathbb{P}_n^U\|_{\mathfrak{I}} \leq \|\mathbb{P}_n^U - \mathbb{P}^U\|_{\mathfrak{I}} + \|\mathbb{P}^U\|_{\mathfrak{I}} = O_p^*(1). \quad (\text{S14})$$

By this result, (S12) and (S13),

$$\frac{1}{n} \sum_{i=1}^n \frac{1}{h^3} K'' \left( \frac{\dot{\Delta}_i - v}{h} \right) (\hat{\Delta}_i - \Delta_i)^2 \mathbb{1}(X_i = x) = O_p^* \left( \frac{\log(n)}{nh^2} \right), \quad (\text{S15})$$

uniformly in  $v \in I_x$ .

By the definition of  $\hat{\Delta}_i$  and  $\Delta_i$ ,

$$\begin{aligned} \frac{1}{n} \sum_{i=1}^n \frac{1}{h^2} K' \left( \frac{\Delta_i - v}{h} \right) (\hat{\Delta}_i - \Delta_i) \mathbb{1}(X_i = x) &= -\frac{1}{n} \sum_{i=1}^n \frac{1}{h^2} K' \left( \frac{\Delta_i - v}{h} \right) D_i \left\{ \hat{\phi}_{0X_i}^{-i}(Y_i) - \phi_{0X_i}^{-i}(Y_i) \right\} \mathbb{1}(X_i = x) \\ &\quad + \frac{1}{n} \sum_{i=1}^n \frac{1}{h^2} K' \left( \frac{\Delta_i - v}{h} \right) (1 - D_i) \left\{ \hat{\phi}_{1X_i}^{-i}(Y_i) - \phi_{1X_i}^{-i}(Y_i) \right\} \mathbb{1}(X_i = x). \end{aligned} \quad (\text{S16})$$

Write

$$\begin{aligned} \frac{1}{n} \sum_{i=1}^n \frac{1}{h^2} K' \left( \frac{\Delta_i - v}{h} \right) \mathbb{1}(D_i = d', X_i = x) \left\{ \hat{\phi}_{dx}^{-i}(Y_i) - \phi_{dx}^{-i}(Y_i) \right\} &= \frac{1}{n} \sum_{i=1}^n \frac{1}{h^2} K' \left( \frac{\Delta_i - v}{h} \right) \mathbb{1}(D_i = d', X_i = x) \\ &\quad \times \left\{ \frac{1}{n-1} \sum_{j \neq i} \mathcal{L}_{dx}(W_j; Y_i) + \hat{\phi}_{dx}^{-i}(Y_i) - \phi_{dx}^{-i}(Y_i) - \frac{1}{n-1} \sum_{j \neq i} \mathcal{L}_{dx}(W_j; Y_i) \right\}. \end{aligned}$$

It is easy to see from the proof of Lemma 1 that (38) also holds for  $\hat{\phi}_{dx}^{-i}(y)$  and the remainder term is uniform

in  $i = 1, \dots, n$ . By Lemma 1 and (S14),

$$\frac{1}{n} \sum_{i=1}^n \frac{1}{h^2} K' \left( \frac{\Delta_i - v}{h} \right) \mathbb{1}(D_i = d', X_i = x) \left\{ \widehat{\phi}_{dx}^{-i}(Y_i) - \phi_{dx}^{-i}(Y_i) - \frac{1}{n-1} \sum_{j \neq i} \mathcal{L}_{dx}(W_j; Y_i) \right\} = O_p^* \left( \frac{\log(n)^{3/4}}{n^{3/4}h} \right),$$

uniformly in  $v \in I_x$ , and therefore

$$\begin{aligned} \frac{1}{n} \sum_{i=1}^n \frac{1}{h^2} K' \left( \frac{\Delta_i - v}{h} \right) (\widehat{\Delta}_i - \Delta_i) \mathbb{1}(X_i = x) &= \\ \frac{1}{n_{(2)}} \sum_{(i,j)} \frac{1}{h^2} K' \left( \frac{\Delta_i - v}{h} \right) \{ (1 - D_i) \mathcal{L}_{1x}(W_j; Y_i) - D_i \mathcal{L}_{0x}(W_j; Y_i) \} \mathbb{1}(X_i = x) &+ O_p^* \left( \frac{\log(n)^{1/2}}{n^{3/4}h} \right) = \\ \frac{1}{n_{(2)}} \sum_{(i,j)} \mathcal{G}_x(W_i, W_j; v) &+ O_p^* \left( \frac{\log(n)^{3/4}}{n^{3/4}h} \right). \quad (\text{S17}) \end{aligned}$$

The conclusion follows from this result, (S11), (S15) and (S16). ■

**Proof of Lemma 3.** By definition, we have

$$\begin{aligned} \mathcal{H}_x^{[1]}(U_i; v) &= \int_{\underline{\epsilon}_x}^{\bar{\epsilon}_x} \frac{1}{h^2} K' \left( \frac{\Delta_x(e) - v}{h} \right) \rho_x(e) \{ \mathbb{1}(\epsilon_i \leq e) - F_{\epsilon|X}(e|x) \} de \\ &\quad \times \left\{ \frac{\mathbb{1}(Z_i = 0, X_i = x)}{p_{0x}} - \frac{\mathbb{1}(Z_i = 1, X_i = x)}{p_{1x}} \right\}, \end{aligned}$$

where

$$\rho_x(e) := \frac{f_{\epsilon DX}(e, 0, x)}{\zeta_{1x}(g(1, x, e))} - \frac{f_{\epsilon DX}(e, 1, x)}{\zeta_{0x}(g(0, x, e))}.$$

Since  $\epsilon$  is independent of  $Z$  given  $X$ ,

$$\begin{aligned} \mathbb{E} \left[ \mathcal{H}_x^{[1]}(U; v)^2 \right] &= \mathbb{E} \left[ \left\{ \int_{\underline{\epsilon}_x}^{\bar{\epsilon}_x} \frac{1}{h^2} K' \left( \frac{\Delta_x(e) - v}{h} \right) \rho_x(e) \{ \mathbb{1}(\epsilon \leq e) - F_{\epsilon|X}(e|x) \} de \right\}^2 \middle| X = x \right] \\ &\quad \times \mathbb{E} \left[ \left\{ \frac{\mathbb{1}(Z = 1)}{p_{1x}} - \frac{\mathbb{1}(Z = 0)}{p_{0x}} \right\}^2 \middle| X = x \right] p_x. \quad (\text{S18}) \end{aligned}$$

Note that

$$\mathbb{E} \left[ \left\{ \frac{\mathbb{1}(Z = 1)}{p_{1x}} - \frac{\mathbb{1}(Z = 0)}{p_{0x}} \right\}^2 \middle| X = x \right] p_x = p_{1x}^{-1} + p_{0x}^{-1}. \quad (\text{S19})$$

Then,

$$\begin{aligned} \mathbb{E} \left[ \left\{ \int_{\underline{\epsilon}_x}^{\bar{\epsilon}_x} \frac{1}{h^2} K' \left( \frac{\Delta_x(e) - v}{h} \right) \rho_x(e) \{ \mathbb{1}(\epsilon \leq e) - F_{\epsilon|X}(e|x) \} de \right\}^2 \middle| X = x \right] &= \\ \mathbb{E} \left[ \left\{ \int_{\underline{\epsilon}_x}^{\bar{\epsilon}_x} \frac{1}{h^2} K' \left( \frac{\Delta_x(e) - v}{h} \right) \rho_x(e) \mathbb{1}(\epsilon \leq e) de \right\}^2 \middle| X = x \right] &- \left\{ \int_{\underline{\epsilon}_x}^{\bar{\epsilon}_x} \frac{1}{h^2} K' \left( \frac{\Delta_x(e) - v}{h} \right) \rho_x(e) F_{\epsilon|X}(e|x) de \right\}^2, \quad (\text{S20}) \end{aligned}$$

and

$$\begin{aligned} \mathbb{E} \left[ \left\{ \int_{\bar{\epsilon}_x}^{\bar{\epsilon}_x} \frac{1}{h^2} K' \left( \frac{\Delta_x(e) - v}{h} \right) \rho_x(e) \mathbb{1}(\epsilon \leq e) de \right\}^2 \middle| X = x \right] = \\ h^{-4} \int_{\bar{\epsilon}_x}^{\bar{\epsilon}_x} \int_{\bar{\epsilon}_x}^{\bar{\epsilon}_x} K' \left( \frac{\Delta_x(e) - v}{h} \right) K' \left( \frac{\Delta_x(e') - v}{h} \right) F_{\epsilon|X}(e \wedge e' | x) \rho_x(e) \rho_x(e') dede' = \\ h^{-4} \sum_{k=1}^m \sum_{j=1}^m \int_{\iota_{x,k-1}}^{\iota_{x,k}} \int_{\iota_{x,j-1}}^{\iota_{x,j}} K' \left( \frac{\Delta_x(e) - v}{h} \right) K' \left( \frac{\Delta_x(e') - v}{h} \right) F_{\epsilon|X}(e \wedge e' | x) \rho_x(e) \rho_x(e') dede'. \quad (\text{S21}) \end{aligned}$$

If  $j > k$ , since  $\iota_{x,k} \leq \iota_{x,j-1}$ ,

$$\begin{aligned} \int_{\iota_{x,k-1}}^{\iota_{x,k}} \int_{\iota_{x,j-1}}^{\iota_{x,j}} K' \left( \frac{\Delta_x(e) - v}{h} \right) K' \left( \frac{\Delta_x(e') - v}{h} \right) F_{\epsilon|X}(e \wedge e' | x) \rho_x(e) \rho_x(e') dede' = \\ \left\{ \int_{\iota_{x,k-1}}^{\iota_{x,k}} K' \left( \frac{\Delta_x(e') - v}{h} \right) F_{\epsilon|X}(e' | x) \rho_x(e') de' \right\} \left\{ \int_{\iota_{x,j-1}}^{\iota_{x,j}} K' \left( \frac{\Delta_x(e) - v}{h} \right) \rho_x(e) de \right\}. \quad (\text{S22}) \end{aligned}$$

Note that  $\Delta_x$  is strictly monotonic on  $[\iota_{x,j-1}, \iota_{x,j}]$ . We assume without loss of generality that the restriction  $\Delta_{x,j}$  is strictly increasing. Since  $I_x$  is an inner closed sub-interval of  $\Delta_{x,j}((\iota_{x,j-1}, \iota_{x,j})) = (\Delta_x(\iota_{x,j-1}), \Delta_x(\iota_{x,j}))$ ,  $v \in I_x$  is an interior point of  $(\Delta_x(\iota_{x,j-1}), \Delta_x(\iota_{x,j}))$ . Let  $\psi_{x,j}(t) := \rho_x(\Upsilon_{x,j}(t)) \Upsilon'_{x,j}(t)$ . By change of variables and mean value expansion,

$$\begin{aligned} \int_{\iota_{x,j-1}}^{\iota_{x,j}} \frac{1}{h^2} K' \left( \frac{\Delta_x(e) - v}{h} \right) \rho_x(e) de &= h^{-1} \int_{\frac{\Delta_x(\iota_{x,j-1}) - v}{h}}^{\frac{\Delta_x(\iota_{x,j}) - v}{h}} K'(u) \rho_x(\Upsilon_{x,j}(hu + v)) \Upsilon'_{x,j}(hu + v) du \\ &= h^{-1} \int_{\frac{\Delta_x(\iota_{x,j-1}) - v}{h}}^{\frac{\Delta_x(\iota_{x,j}) - v}{h}} K'(u) \{ \psi_{x,j}(v) + \psi'_{x,j}(\dot{v}) hu \} du, \end{aligned}$$

where the mean value  $\dot{v}$  depends on  $u$  and satisfies  $|\dot{v} - v| \leq h|u|$ . Note that  $\int K'(u) du = 0$ ,  $K'$  is supported on  $[-1, 1]$  and therefore,  $\int_{(\Delta_x(\iota_{x,j-1}) - v)/h}^{(\Delta_x(\iota_{x,j}) - v)/h} K'(u) du = 0$ ,  $\forall v \in I_x$ , when  $h$  is sufficiently small. Therefore,

$$\left| \int_{\iota_{x,j-1}}^{\iota_{x,j}} \frac{1}{h^2} K' \left( \frac{\Delta_x(e) - v}{h} \right) \rho_x(e) de \right| \lesssim \sup_{t \in [\Delta_x(\iota_{x,j-1}), \Delta_x(\iota_{x,j})]} |\psi'_{x,j}(t)|, \quad (\text{S23})$$

uniformly in  $v \in I_x$ , when  $h$  is sufficiently small. Denote  $\chi_{x,j}(t) := F_{\epsilon|X}(\Upsilon_{x,j}(t) | x) \psi_{x,j}(t)$ . Similarly,

$$\left| \int_{\iota_{x,k-1}}^{\iota_{x,k}} \frac{1}{h^2} K' \left( \frac{\Delta_x(e') - v}{h} \right) F_{\epsilon|X}(e' | x) \rho_x(e') de' \right| \lesssim \sup_{t \in [\Delta_x(\iota_{x,k-1}), \Delta_x(\iota_{x,k})]} |\chi'_{x,k}(t)|, \quad (\text{S24})$$

uniformly in  $v \in I_x$ , when  $h$  is sufficiently small. Then, it follows that

$$\begin{aligned} \mathbb{E} \left[ \left\{ \int_{\bar{\epsilon}_x}^{\bar{\epsilon}_x} \frac{1}{h^2} K' \left( \frac{\Delta_x(e) - v}{h} \right) \rho_x(e) \mathbb{1}(\epsilon \leq e) de \right\}^2 \middle| X = x \right] = \\ h^{-4} \sum_{j=1}^m \int_{\iota_{x,j-1}}^{\iota_{x,j}} \int_{\iota_{x,j-1}}^{\iota_{x,j}} K' \left( \frac{\Delta_x(e) - v}{h} \right) K' \left( \frac{\Delta_x(e') - v}{h} \right) F_{\epsilon|X}(e \wedge e' | x) \rho_x(e) \rho_x(e') dede' + O(1). \quad (\text{S25}) \end{aligned}$$

By change of variables,

$$\begin{aligned}
& h^{-4} \int_{\iota_{x,j-1}}^{\iota_{x,j}} \int_{\iota_{x,j-1}}^{\iota_{x,j}} K' \left( \frac{\Delta_x(e) - v}{h} \right) K' \left( \frac{\Delta_x(e') - v}{h} \right) F_{\epsilon|X}(e \wedge e'|x) \rho_x(e) \rho_x(e') \mathrm{d}e \mathrm{d}e' = \\
& h^{-2} \int_{\frac{\Delta_x(\iota_{x,j-1}) - v}{h}}^{\frac{\Delta_x(\iota_{x,j}) - v}{h}} \int_{\frac{\Delta_x(\iota_{x,j-1}) - v}{h}}^{\frac{\Delta_x(\iota_{x,j}) - v}{h}} K'(u) K'(w) F_{\epsilon|X}(\mathcal{I}_{x,j}(hu+v) \wedge \mathcal{I}_{x,j}(hw+v)|x) \\
& \quad \times \rho_x(\mathcal{I}_{x,j}(hu+v)) \mathcal{I}'_{x,j}(hu+v) \rho_x(\mathcal{I}_{x,j}(hw+v)) \mathcal{I}'_{x,j}(hw+v) \mathrm{d}u \mathrm{d}w = \\
& \quad 2h^{-2} \int K'(w) \psi_{x,j}(hw+v) \left\{ \int_{-\infty}^w K'(u) \chi_{x,j}(hu+v) \mathrm{d}u \right\} \mathrm{d}w, \quad (\text{S26})
\end{aligned}$$

where the second equality follows from symmetry and holds when  $h$  is sufficiently small. By integration by parts,

$$\int_{-\infty}^w K'(u) \chi_{x,j}(hu+v) \mathrm{d}u = K(w) \chi_{x,j}(hw+v) - h \int_{-\infty}^w K(u) \chi'_{x,j}(hu+v) \mathrm{d}u. \quad (\text{S27})$$

Then,

$$\begin{aligned}
& h^{-1} \int K'(w) K(w) \{ \psi_{x,j}(hw+v) \chi_{x,j}(hw+v) - \psi_{x,j}(v) \chi_{x,j}(v) \\
& \quad - (\psi'_{x,j}(v) \chi_{x,j}(v) + \psi_{x,j}(v) \chi'_{x,j}(v)) hw \} \mathrm{d}w = \int K'(w) K(w) w \{ (\psi'_{x,j}(\dot{v}) \chi_{x,j}(\dot{v}) + \psi_{x,j}(\dot{v}) \chi'_{x,j}(\dot{v})) \\
& \quad - (\psi'_{x,j}(v) \chi_{x,j}(v) + \psi_{x,j}(v) \chi'_{x,j}(v)) \} \mathrm{d}w = o(1), \quad (\text{S28})
\end{aligned}$$

where the mean value  $\dot{v}$  depends on  $u$  and satisfies  $|\dot{v} - v| \leq h|u|$  and the second equality holds uniformly in  $v \in I_x$ . Similarly,

$$\begin{aligned}
& \int K'(w) \psi_{x,j}(hw+v) \left( \int_{-\infty}^w K(u) \chi'_{x,j}(hu+v) \mathrm{d}u \right) \mathrm{d}w - \psi_{x,j}(v) \chi'_{x,j}(v) \int K'(w) \left( \int_{-\infty}^w K(u) \mathrm{d}u \right) \mathrm{d}w = \\
& \int \int_{-\infty}^w K'(w) K(u) \{ \psi_{x,j}(hw+v) \chi'_{x,j}(hu+v) - \psi_{x,j}(v) \chi'_{x,j}(v) \} \mathrm{d}u \mathrm{d}w = o(1), \quad (\text{S29})
\end{aligned}$$

the second equality holds uniformly in  $v \in I_x$ . By integration by parts,  $\int K'(w) \left( \int_{-\infty}^w K(u) \mathrm{d}u \right) \mathrm{d}w = - \int K(u)^2 \mathrm{d}u$  and  $\int K'(w) K(w) w \mathrm{d}w = \left( - \int K(u)^2 \mathrm{d}u \right) / 2$ . Now it follows from these equalities, (S26), (S27), (S28) and (S29) that

$$\begin{aligned}
& h^{-3} \int_{\iota_{x,j-1}}^{\iota_{x,j}} \int_{\iota_{x,j-1}}^{\iota_{x,j}} K' \left( \frac{\Delta_x(e) - v}{h} \right) K' \left( \frac{\Delta_x(e') - v}{h} \right) F_{\epsilon|X}(e \wedge e'|x) \rho_x(e) \rho_x(e') \mathrm{d}e \mathrm{d}e' = \\
& \quad 2 (\psi'_{x,j}(v) \chi_{x,j}(v) + \psi_{x,j}(v) \chi'_{x,j}(v)) \int K'(w) K(w) w \mathrm{d}w \\
& \quad - 2 \psi_{x,j}(v) \chi'_{x,j}(v) \int K'(w) \left( \int_{-\infty}^w K(u) \mathrm{d}u \right) \mathrm{d}w + o(1) = (\psi_{x,j}(v) \chi'_{x,j}(v) - \psi'_{x,j}(v) \chi_{x,j}(v)) \int K(u)^2 \mathrm{d}u + o(1), \quad (\text{S30})
\end{aligned}$$

uniformly in  $v \in I_x$ . Note that

$$\psi_{x,j}(v) \chi'_{x,j}(v) - \psi'_{x,j}(v) \chi_{x,j}(v) = \left\{ \frac{f_{\epsilon DX}(\mathcal{I}_{x,j}(v), 0, x)}{\zeta_{1x}(g(1, x, \mathcal{I}_{x,j}(v)))} - \frac{f_{\epsilon DX}(\mathcal{I}_{x,j}(v), 1, x)}{\zeta_{0x}(g(0, x, \mathcal{I}_{x,j}(v)))} \right\}^2 f_{\epsilon|X}(\mathcal{I}_{x,j}(v)|x) \mathcal{I}'_{x,j}(v)^3.$$

Now it follows from this equality, (S18), (S19), (S20), (S25) and (S30) that  $\mathbb{E} \left[ \mathcal{H}_x^{[1]}(U; v)^2 \right] = h^{-1} \mathcal{V}_{\Delta X}^\dagger(v, x) + o(h^{-1})$ , uniformly in  $v \in I_x$ . Denote  $\mathfrak{H} := \{\mathcal{H}_x(\cdot; v) : v \in I_x\}$  and  $\mathfrak{H}^{[1]} := \{\mathcal{H}_x^{[1]}(\cdot; v) : v \in I_x\}$ . Therefore, we have  $\sigma_{\mathfrak{H}^{[1]}}^2 := \sup_{f \in \mathfrak{H}^{[1]}} \mathbb{P}^U f^2 = O(h^{-1})$ . By law of iterated expectations,

$$\begin{aligned} \mathbb{E} \left[ \mathcal{H}_x(U_1, U_2; v)^2 \right] &= \\ \mathbb{E} \left[ \frac{1}{h^4} K' \left( \frac{\Delta_x(\epsilon) - v}{h} \right)^2 \left\{ \frac{\mathbb{1}(D=0, X=x)}{\zeta_{1x}(g(1, x, \epsilon))^2} + \frac{\mathbb{1}(D=1, X=x)}{\zeta_{1x}(g(0, x, \epsilon))^2} \right\} F_{\epsilon|X}(\epsilon|x) (1 - F_{\epsilon|X}(\epsilon|x)) \right] & \\ &= O(h^{-3}), \quad (\text{S31}) \end{aligned}$$

uniformly in  $v \in I_x$ . Therefore,  $\sigma_{\mathfrak{H}}^2 := \sup_{f \in \mathfrak{H}} \mathbb{P}^{(2)} f^2 = O(h^{-3})$ .

Since  $\|K''\|_{\mathbb{R}} < \infty$ , where we denote  $\|K''\|_{\mathbb{R}} := \sup_{u \in \mathbb{R}} |K''(u)|$ , the restriction of  $K'$  on  $[-1, 1]$  is of bounded variation. There exists a decomposition  $K' = L_1 - L_2$ , where  $L_1$  and  $L_2$  are non-decreasing and bounded. It follows from Kosorok (2007, Lemma 9.6) that  $\{(\Delta_x(\cdot) - v)/h : v \in I_x\}$  is VC-subgraph with VC index being at most 4,  $\forall h > 0$ . Then, by Kosorok (2007, Lemma 9.9(viii)),  $\mathfrak{C}_k := \{h^{-2} L_k((\Delta_x(\cdot) - v)/h) : v \in I_x\}$  is VC-subgraph with VC index being at most 4,  $\forall h > 0$ , and by Kosorok (2007, Lemma 9.9(vi)), each of  $\mathfrak{C}_1 \cdot \mathcal{C}_x$  and  $\mathfrak{C}_2 \cdot \mathcal{C}_x$  is VC-subgraph with VC index being at most 7,  $\forall h > 0$ , with a constant envelope that is a multiple of  $h^{-2}$  (under Assumption 4(c)). Then,  $\mathfrak{H}$  can be written as (a sub-class of) the pointwise difference of  $\mathfrak{C}_1 \cdot \mathcal{C}_x$  and  $\mathfrak{C}_2 \cdot \mathcal{C}_x$ . Then, by Giné and Nickl (2016, Theorem 3.6.9) and Chernozhukov et al. (2014, Lemma A.6),  $\mathfrak{H}$  is uniformly VC-type with respect to a constant envelope  $F_{\mathfrak{H}} \propto h^{-2}$ .

For a VC-type class  $\mathfrak{F}$  of functions defined on  $\mathcal{S}_U$  with respect to an envelope  $F_{\mathfrak{F}}$  (assume that  $\mathfrak{F}$  is centered:  $\mathbb{P}^U f = 0, \forall f \in \mathfrak{F}$ ), by standard calculations (see, e.g., the proof of Chernozhukov et al., 2014, Corollary 5.1) and Chernozhukov et al. (2014, Lemma 2.1), there exists a zero-mean Gaussian process  $\{G^U(f) : f \in \mathfrak{F}\}$  that is a tight random element in  $\ell^\infty(\mathfrak{F})$  and has the same covariance structure as the empirical process  $\{\mathbb{G}_n^U f : f \in \mathfrak{F}\}$  (i.e.,  $\mathbb{E}[G^U(f) G^U(g)] = \mathbb{E}[f(U) g(U)], \forall f, g \in \mathfrak{F}$ ). The tightness of  $\mathfrak{F}$  is equivalent to the condition that  $\mathfrak{F}$  (endowed with the intrinsic pseudo metric  $\mathfrak{F}^2 \ni (f, g) \mapsto \sqrt{\mathbb{E}[(G^U(f) - G^U(g))^2]} = \|f - g\|_{\mathbb{P}^U, 2}$ ) is totally bounded and almost surely the sample paths  $f \mapsto G^U(f)$  are uniformly continuous with respect to the intrinsic pseudo metric (therefore,  $\Pr[\|G^U\|_{\mathfrak{F}} < \infty] = 1$ ). And  $\{G^U(f) : f \in \mathfrak{F}\}$  is also separable as a stochastic process. See Kosorok (2007, Lemmas 7.2 and 7.4). Since  $F_{\mathfrak{F}}$  is also an envelope of  $\mathfrak{F}_\pm := \mathfrak{F} \cup (-\mathfrak{F})$  and the covering number of  $\mathfrak{F}_\pm$  is at most twice that of  $\mathfrak{F}$ ,  $\mathfrak{F}_\pm$  is VC-type with respect to  $F_{\mathfrak{F}}$  and therefore, there exists a zero-mean Gaussian process  $\{G^U(f) : f \in \mathfrak{F}_\pm\}$  that is a tight random element in  $\ell^\infty(\mathfrak{F}_\pm)$  and has the same covariance structure as that of  $\{\mathbb{G}_n^U f : f \in \mathfrak{F}_\pm\}$ . Moreover, by Giné and Nickl (2016, Theorem 3.7.28), almost surely the sample paths  $\mathfrak{F}_\pm \ni f \mapsto G^U(f)$  are prelinear and therefore, almost surely,  $\forall f \in \mathfrak{F}, G^U(f) + G^U(-f) = 0$ , and  $\sup_{f \in \mathfrak{F}_\pm} G^U(f) = \|G^U\|_{\mathfrak{F}}$ . In our first application,  $\mathfrak{F} = \mathfrak{H}^{[1]}$ , which is also uniformly VC-type (by Lemma A.3 of CK) with respect to the constant envelope  $F_{\mathfrak{H}^{[1]}} = F_{\mathfrak{H}}$ .

By the coupling theorem (CK Proposition 2.1 with  $\mathcal{H} = \mathfrak{H}_\pm, \bar{\sigma}_{\mathfrak{g}} = \sigma_{\mathfrak{H}^{[1]}}, \sigma_{\mathfrak{h}} = \sigma_{\mathfrak{H}}, b_{\mathfrak{g}} = b_{\mathfrak{h}} = F_{\mathfrak{H}}, \gamma = \sqrt{\log(n)/(nh^3)}$  and  $q = \infty$ ), one can construct a coupling  $(Z_{\mathfrak{H}_\pm}, \tilde{Z}_{\mathfrak{H}_\pm})$  that satisfies the following conditions:  $Z_{\mathfrak{H}_\pm} := \sup_{f \in \mathfrak{H}_\pm} \mathbb{U}_n^{(2)} f = \|\mathbb{U}_n^{(2)}\|_{\mathfrak{H}_\pm}, \tilde{Z}_{\mathfrak{H}_\pm} = \sup_{f \in \mathfrak{H}_\pm^{[1]}} G^U(f) = \|G^U\|_{\mathfrak{H}^{[1]}}$ , where  $\{G^U(f) : f \in \mathfrak{H}_\pm^{[1]}\}$  has the same covariance structure as that of the (Hájek) empirical process  $\{\mathbb{G}_n f : f \in \mathfrak{H}_\pm^{[1]}\}$ , and  $(Z_{\mathfrak{H}_\pm}, \tilde{Z}_{\mathfrak{H}_\pm})$  satisfies  $Z_{\mathfrak{H}_\pm} - \tilde{Z}_{\mathfrak{H}_\pm} = O_p^*\left(\sqrt{\log(n)/h}, \sqrt{\log(n)/(nh^3)}\right)$ . By Dudley's entropy integral bound (Giné and Nickl, 2016, Theorem 2.3.7), Lemma A.2 of CK, (37) and standard calculations (see, e.g., calculations in the proof of Chernozhukov

et al., 2014, Corollary 5.1),

$$\begin{aligned}
\mathbb{E} \left[ \|G^U\|_{\mathfrak{H}^{[1]}} \right] &\lesssim \int_0^{\sigma_{\mathfrak{H}^{[1]}} \vee n^{-1/2} \|F_{\mathfrak{H}^{[1]}}\|_{\mathbb{P}^U, 2}} \sqrt{1 + \log \left( N \left( \epsilon, \mathfrak{H}^{[1]}, \|\cdot\|_{\mathbb{P}^U, 2} \right) \right)} d\epsilon \\
&\leq 4 \|F_{\mathfrak{H}^{[1]}}\|_{\mathbb{P}^U, 2} \int_0^{\frac{\sigma_{\mathfrak{H}^{[1]}} \vee n^{-1/2} \|F_{\mathfrak{H}^{[1]}}\|_{\mathbb{P}^U, 2}}{4 \|F_{\mathfrak{H}^{[1]}}\|_{\mathbb{P}^U, 2}}} \sqrt{1 + \log \left( \sup_{Q \in \mathcal{Q}_{\mathcal{H}^d}^{\text{td}}} N \left( \epsilon \|F_{\mathfrak{H}^{[1]}}\|_{Q, 2}, \mathfrak{H}^{[1]}, \|\cdot\|_{Q, 2} \right) \right)} d\epsilon \\
&\lesssim \left( \sigma_{\mathfrak{H}^{[1]}} \vee n^{-1/2} \|F_{\mathfrak{H}^{[1]}}\|_{\mathbb{P}^U, 2} \right) \sqrt{\log(n)},
\end{aligned}$$

when  $n$  is sufficiently large. By the Borell-Sudakov-Tsirelson inequality (Giné and Nickl, 2016, Theorem 2.5.8),  $\Pr \left[ \|G^U\|_{\mathfrak{H}^{[1]}} \geq \mathbb{E} \left[ \|G^U\|_{\mathfrak{H}^{[1]}} \right] + \sqrt{2 \cdot \log(n)} \sigma_{\mathfrak{H}^{[1]}} \right] \leq n^{-1}$ . Therefore, since  $\tilde{Z}_{\mathfrak{H}^\pm} =_d \|G^U\|_{\mathfrak{H}^{[1]}}$ , we have  $\tilde{Z}_{\mathfrak{H}^\pm} = O_p^* \left( \sqrt{\log(n)/h} \right)$  and  $Z_{\mathfrak{H}^\pm} = \left\| \mathbb{U}_n^{(2)} \right\|_{\mathfrak{H}} = O_p^* \left( \sqrt{\log(n)/h}, \sqrt{\log(n)/(nh^3)} \right)$ . The conclusion follows from these results.  $\blacksquare$

## S2 Proofs of Lemmas 4, 5 and 6

**Proof of Lemma 4.** Denote  $\Pi_{dx}(y) := \Pi_{d1x}(y) + \Pi_{d0x}(y)$  and  $\hat{\Pi}_{dx}(y) := \hat{\Pi}_{d1x}(y) + \hat{\Pi}_{d0x}(y)$ . Then,  $\hat{R}_{d'x}(y) = \left( \hat{\Pi}_{dx}(\hat{\phi}_{dx}(y)) + \hat{\Pi}_{d'x}(y) \right) / \hat{p}_x$  and  $R_{d'x}(y) = \left( \Pi_{dx}(\phi_{dx}(y)) + \Pi_{d'x}(y) \right) / p_x$ . Part (a) follows from the following facts:  $\left\| \hat{\Pi}_{dx} \circ \hat{\phi}_{dx} - \Pi_{dx} \circ \phi_{dx} \right\|_{I_{d'x}} = O_p^* \left( \sqrt{\log(n)/n} \right)$ ,  $\left\| \hat{\Pi}_{d'x} - \Pi_{d'x} \right\|_{I_{d'x}} = O_p^* \left( \sqrt{\log(n)/n} \right)$  and  $\hat{p}_x - p_x = O_p^* \left( \sqrt{\log(n)/n} \right)$ . Part (b) follows from similar arguments used to show  $\left\| \mathbb{P}_n^U - \mathbb{P}^U \right\|_{\mathfrak{J}} = O_p^* \left( \sqrt{\log(n)/(nh)} \right)$  in the proof of Lemma 2,  $\hat{p}_{z|x} - p_{z|x} = O_p^* \left( \sqrt{\log(n)/n} \right)$ , Abadie (2003, Theorem 3.1) and standard arguments for the bias of kernel density estimators.  $\blacksquare$

**Proof of Lemma 5.** By definition, we have  $\Pr[Y_n > C_2 \alpha_n] \leq C_3 \beta_n$  and  $\Pr[\Pr_{|W_1^n} [|X_n| > C_1 Y_n] > C_4 \gamma_n] \leq C_5 \delta_n$ . Part (a) follows from

$$1 - C_3 \beta_n - C_5 \delta_n \leq \Pr[Y_n \leq C_2 \alpha_n, \Pr_{|W_1^n} [|X_n| > C_1 Y_n] \leq C_4 \gamma_n] \leq \Pr[\Pr_{|W_1^n} [|X_n| > C_1 C_2 \alpha_n] \leq C_4 \gamma_n].$$

Part (b) follows from

$$\Pr[\Pr_{|W_1^n} [|Y_n| > C_2 \alpha_n] > \epsilon_n] = \Pr[\mathbb{1}(|Y_n| > C_2 \alpha_n) > \epsilon_n] = \Pr[|Y_n| > C_2 \alpha_n] \leq C_3 \beta_n.$$

**Proof of Lemma 6.** Denote  $S^\sharp(v, x) := p_x S^\sharp(v|x)$ ,  $\hat{S}^\sharp(v, x) := \hat{p}_x \hat{S}^\sharp(v|x)$ ,  $\pi_i := \mathbb{1}(Z_i = 0, X_i = x) / p_{0x} - \mathbb{1}(Z_i = 1, X_i = x) / p_{1x}$  and  $\hat{\pi}_i := \mathbb{1}(Z_i = 0, X_i = x) / \hat{p}_{0x} - \mathbb{1}(Z_i = 1, X_i = x) / \hat{p}_{1x}$ . Then, we write

$$\begin{aligned}
\hat{S}^\sharp(v, x) - S^\sharp(v, x) &= \frac{1}{\sqrt{n}} \sum_{i=1}^n \nu_i \left\{ \hat{\mathcal{U}}_x^{[1]}(W_i; v) - \tilde{\mathcal{U}}_x^{[1]}(W_i; v) \right\} - \left( \frac{1}{\sqrt{n}} \sum_{i=1}^n \nu_i \right) (\hat{\mu}_{\mathcal{U}_x}(v) - \tilde{\mu}_{\mathcal{U}_x}(v)) \\
&\quad - \frac{1}{\sqrt{n}} \sum_{i=1}^n \nu_i \left\{ \tilde{\mathcal{U}}_x^{[2]}(W_i; v) - \tilde{\mu}_{\mathcal{U}_x}(v) \right\}. \quad (\text{S32})
\end{aligned}$$

By Taylor expansion,

$$\begin{aligned}
& \frac{1}{\sqrt{n}} \sum_{i=1}^n \nu_i \left\{ \widehat{\mathcal{U}}_x^{[1]}(W_i; v) - \widetilde{\mathcal{U}}_x^{[1]}(W_i; v) \right\} = \\
& \frac{1}{\sqrt{n}} \sum_{i=1}^n \nu_i h^{-3/2} M' \left( \frac{\Delta_i - v}{h} \right) (\widehat{\Delta}_i - \Delta_i) \mathbb{1}(X_i = x) + \frac{1}{2} \frac{1}{\sqrt{n}} \sum_{i=1}^n \nu_i h^{-5/2} M'' \left( \frac{\Delta_i - v}{h} \right) (\widehat{\Delta}_i - \Delta_i)^2 \mathbb{1}(X_i = x) \\
& + \frac{1}{\sqrt{n}} \sum_{i=1}^n \nu_i \left\{ \frac{1}{n-1} \sum_{j \neq i} h^{-3/2} M' \left( \frac{\widehat{\Delta}_j - v}{h} \right) (\widehat{q}_x(W_j, W_i) \widehat{\pi}_i - q_x(W_j, W_i) \pi_i) \right\} \\
& + \frac{1}{\sqrt{n}} \sum_{i=1}^n \nu_i \left\{ \frac{1}{n-1} \sum_{j \neq i} h^{-3/2} \left( M' \left( \frac{\widehat{\Delta}_j - v}{h} \right) - M' \left( \frac{\Delta_j - v}{h} \right) \right) q_x(W_j, W_i) \pi_i \right\} \\
& =: T_1^\sharp(v) + T_2^\sharp(v) + T_3^\sharp(v) + T_4^\sharp(v),
\end{aligned}$$

where  $\widehat{\Delta}_i$  denotes the mean value that lies between  $\Delta_i$  and  $\widehat{\Delta}_i$ . By the concentration inequality for the maximum of normal random variables (e.g., [Giné and Nickl, 2016](#), (2.3)) and  $\mathbb{E}[\max_{1 \leq i \leq n} |\nu_i|] \lesssim \sqrt{\log(n)}$  ([Giné and Nickl, 2016](#), Lemma 2.4.11),  $\Pr_{|W_1^n} \left[ \max_{1 \leq i \leq n} |\nu_i| > C_1 \sqrt{\log(n)} \right] \leq 2n^{-1}$ . Denote  $N_j(v) := \mathbb{1}(|\Delta_j - v| \leq 2h) + \varsigma^3 \mu_{K,2} \mathbb{1}(|\Delta_j - v| \leq 2h_b)$ . Let  $\overline{N}_x(v) := (nh)^{-1} \sum_{j=1}^n N_j(v) \mathbb{1}(X_j = x)$ . Then it follows from arguments used to show (S14) that  $\overline{N}_x(v) = O_p^*(1)$  uniformly in  $v \in I_x$ . Then, by Lemma 5, (S12) and  $\|T_2^\sharp\|_{I_x} \lesssim \sqrt{n} h^{-3/2} \left( \max_{1 \leq i \leq n} |\nu_i| \right) \times \|\overline{N}_x\|_{I_x} \overline{\Delta}^2$ , we have  $\|T_2^\sharp\|_{I_x} = O_p^* \left( \sqrt{\log(n)^3 / (nh^3)} \right)$ .

Let  $s_i(v) := h^{-3/2} M'((\Delta_i - v)/h) (\widehat{\Delta}_i - \Delta_i) \mathbb{1}(X_i = x)$ . Denote  $S := \{(s_1(v), \dots, s_n(v)) \in \mathbb{R}^n : v \in I_x\}$ . Then  $\|T_1^\sharp\|_{I_x} = \sup_{(s_1, \dots, s_n) \in S} |n^{-1/2} \sum_{i=1}^n \nu_i s_i|$ , where  $\{n^{-1/2} \sum_{i=1}^n \nu_i s_i : (s_1, \dots, s_n) \in S \cup \{0\}\}$  is a centered Gaussian process, conditionally on the data. Let  $\|\cdot\|_{n,2}$  be the implicit norm on  $S$  induced by the Gaussian process:  $\|(s_1, \dots, s_n)\|_{n,2} := \sqrt{\mathbb{E}_{|W_1^n} \left[ \left( n^{-1/2} \sum_{i=1}^n \nu_i s_i \right)^2 \right]} = \sqrt{n^{-1} \sum_{i=1}^n s_i^2}$ . It is easy to see  $\sqrt{n^{-1} \sum_{i=1}^n (s_i(v) - s_i(v'))^2} \leq C_M h^{-5/2} \overline{\Delta} |v - v'|$ , where  $C_M := \|K''\|_{\mathbb{R}} + \varsigma^5 \mu_{K,2} \|K_b^{(4)}\|_{\mathbb{R}}$  and  $K_b^{(4)}$  denotes the fourth derivative of  $K_b$ . Therefore,  $N(\epsilon \cdot C_M h^{-5/2} \overline{\Delta}, S, \|\cdot\|_{n,2}) \leq N(\epsilon, I_x, |\cdot|) \leq 1 + |I_x|/\epsilon$ , where  $|I_x|$  denotes the length of  $I_x$ . Let  $\sigma_n^2 := \sup_{(s_1, \dots, s_n) \in S} \|(s_1, \dots, s_n)\|_{n,2}^2 = \sup_{v \in I_x} \mathbb{E}_{|W_1^n} [T_1^\sharp(v)^2]$  and then,

$$\sigma_n \leq \overline{\Delta} \sqrt{\sup_{v \in I_x} \frac{1}{n} \sum_{i=1}^n h^{-3} M' \left( \frac{\Delta_i - v}{h} \right)^2} = O_p^* \left( \sqrt{\frac{\log(n)}{nh^2}} \right), \quad (\text{S33})$$

where the last equality follows from (S12). By Dudley's metric entropy bound ([Giné and Nickl, 2016](#), Theorem 2.3.7), the above inequality and standard calculations,

$$\begin{aligned}
\mathbb{E}_{|W_1^n} \left[ \left\| T_1^\sharp \right\|_{I_x} \right] & \lesssim \int_0^{\sigma_n \vee n^{-1/2} C_M h^{-5/2} \overline{\Delta}} \sqrt{1 + \log \left( N(\epsilon, S, \|\cdot\|_{n,2}) \right)} d\epsilon \\
& \leq \left( C_M h^{-5/2} \overline{\Delta} \right) \int_0^{\frac{\sigma_n \vee n^{-1/2} C_M h^{-5/2} \overline{\Delta}}{C_M h^{-5/2} \overline{\Delta}}} \sqrt{1 + \log \left( N(\epsilon, I_x, |\cdot|) \right)} d\epsilon \\
& \lesssim \left( \sigma_n \vee n^{-1/2} C_M h^{-5/2} \overline{\Delta} \right) \sqrt{\log(|I_x| n^{1/2})}, \quad (\text{S34})
\end{aligned}$$

when  $n$  is sufficiently large. Then, by the Borell-Sudakov-Tsirelson concentration inequality ([Giné and Nickl, 2016](#), Theorem 2.5.8),  $\Pr_{|W_1^n} \left[ \left\| T_1^\sharp \right\|_{I_x} > \mathbb{E}_{|W_1^n} \left[ \left\| T_1^\sharp \right\|_{I_x} \right] + \sigma_n \sqrt{2 \cdot \log(n)} \right] \leq n^{-1}$ . By Lemma 5, (S33) and (S34),

$$\|T_1^\sharp\|_{I_x} = O_p^\sharp(\log(n)/\sqrt{nh^2}).$$

Denote  $\varphi_{dx}(W_j, W_i) := \mathbb{1}(Y_i \leq \phi_{dx}(Y_j), D_i = d) + \mathbb{1}(Y_i \leq Y_j, D_i = d') - R_{d'x}(Y_j)$  and  $\widehat{\varphi}_{dx}(W_j, W_i) := \mathbb{1}(Y_i \leq \widehat{\phi}_{dx}(Y_j), D_i = d) + \mathbb{1}(Y_i \leq Y_j, D_i = d') - \widehat{R}_{d'x}(Y_j)$ . Then, by (S4),

$$\begin{aligned} \widehat{q}_{dx}(W_j, W_i) - q_{dx}(W_j, W_i) &= \mathbb{1}(D_j = d', X_j = x) \left\{ \frac{\widehat{\varphi}_{dx}(W_j, W_i)}{\widehat{\zeta}_{dx}(\phi_{dx}(Y_j))} - \frac{\varphi_{dx}(W_j, W_i)}{\zeta_{dx}(\phi_{dx}(Y_j))} \right. \\ &\quad \left. - \frac{\widehat{\varphi}_{dx}(W_j, W_i) \left( \widehat{\zeta}_{dx}(\widehat{\phi}_{dx}(Y_j)) - \zeta_{dx}(\phi_{dx}(Y_j)) \right)}{\widehat{\zeta}_{dx}(\phi_{dx}(Y_j))^2} + \frac{\widehat{\varphi}_{dx}(W_j, W_i) \left( \widehat{\zeta}_{dx}(\widehat{\phi}_{dx}(Y_j)) - \zeta_{dx}(\phi_{dx}(Y_j)) \right)^2}{\widehat{\zeta}_{dx}(\widehat{\phi}_{dx}(Y_j)) \zeta_{dx}(\phi_{dx}(Y_j))^2} \right\}. \end{aligned} \quad (\text{S35})$$

Write

$$T_3^\sharp(v) = \frac{1}{\sqrt{n(2)}} \sum_{j=1}^n h^{-3/2} M' \left( \frac{\widehat{\Delta}_j - v}{h} \right) \frac{1}{\sqrt{n-1}} \sum_{i \neq j} \nu_i (\widehat{q}_x(W_j, W_i) \widehat{\pi}_i - q_x(W_j, W_i) \pi_i).$$

Then, in view of (S12), with probability at least  $1 - C_2 n^{-1}$ ,  $\|T_3^\sharp\|_{I_x} \leq \sqrt{n/(n-1)} h^{-1/2} \|\overline{N}_x\|_{I_x} \max_{1 \leq j \leq n} |\Xi_j|$ , where

$$\Xi_j := \frac{1}{\sqrt{n-1}} \sum_{i \neq j} \nu_i \mathbb{1}(\Delta_j \in I_x^{2h \vee h_b}) (\widehat{q}_x(W_j, W_i) \widehat{\pi}_i - q_x(W_j, W_i) \pi_i)$$

and  $I_x^{2h \vee h_b}$  denotes the  $2h \vee h_b$  enlargement of  $I_x$ . Conditionally on the data  $(W_1^n)$ ,  $(\Xi_1, \dots, \Xi_n)$  are centered and jointly normal. Then, by the  $c_r$  inequality,

$$\begin{aligned} \mathbb{E}_{|W_1^n} [\Xi_j^2] &\leq \sum_{d \in \{0,1\}} \frac{1}{n-1} \sum_{i \neq j} (\widehat{q}_{dx}(W_j, W_i) - q_{dx}(W_j, W_i))^2 \pi_i^2 + \frac{1}{n-1} \sum_{i \neq j} \widehat{q}_x(W_j, W_i)^2 (\widehat{\pi}_i - \pi_i)^2 \\ &=: T_{1,j}^\Xi + T_{2,j}^\Xi \end{aligned}$$

It can be shown that  $\max_{1 \leq j \leq n} |T_{2,j}^\Xi| = O_p^\star(\log(n)/n)$ . By Lemma 4 and (S3),

$$\widehat{\zeta}_{dx}(\widehat{\phi}_{dx}(y)) - \zeta_{dx}(\phi_{dx}(y)) = O_p^\star \left( \sqrt{\frac{\log(n)}{nh_g}} + h_g^2 \right), \quad (\text{S36})$$

uniformly in  $y \in \dot{I}_{d'x}$ , where  $\dot{I}_{d'x}$  is any closed sub-interval of  $I_{d'x}$ . (S36) implies that  $\inf_{y \in \dot{I}_{d'x}} |\widehat{\zeta}_{dx}(\widehat{\phi}_{dx}(y))| > \inf_{y \in \dot{I}_{d'x}} |\zeta_{dx}(\phi_{dx}(y))|/2$  with probability greater than  $1 - C_2 n^{-1}$  when  $n$  is sufficiently large. And, by this result, (S35) and (S36),

$$\begin{aligned} \frac{1}{n-1} \sum_{i \neq j} (\widehat{q}_{dx}(W_j, W_i) - q_{dx}(W_j, W_i))^2 \pi_i^2 &= \\ &= \frac{\mathbb{1}(D_j = d', X_j = x)}{\widehat{\zeta}_{dx}(\phi_{dx}(Y_j))^2} \frac{1}{n-1} \sum_{i \neq j} (\widehat{\varphi}_{dx}(W_j, W_i) - \varphi_{dx}(W_j, W_i))^2 \pi_i^2 + O_p^\star \left( \frac{\log(n)}{nh_g} + h_g^4 \right) = \\ &= \frac{\mathbb{1}(D_j = d', X_j = x)}{\zeta_{dx}(\phi_{dx}(Y_j))^2} \frac{1}{n-1} \sum_{i \neq j} \left\{ \mathbb{1}(Y_i \leq \widehat{\phi}_{dx}(Y_j)) - \mathbb{1}(Y_i \leq \phi_{dx}(Y_j)) \right\}^2 \mathbb{1}(D_i = d) \pi_i^2 + O_p^\star \left( \frac{\log(n)}{nh_g} + h_g^4 \right). \end{aligned}$$

In view of (S3), with probability at least  $1 - C_2 n^{-1}$ ,

$$\sup_{y \in \dot{I}_{d'x}} \left| \frac{1}{n} \sum_{i=1}^n \left\{ \mathbb{1}(Y_i \leq \widehat{\phi}_{dx}(y)) - \mathbb{1}(Y_i \leq \phi_{dx}(y)) \right\}^2 \mathbb{1}(D_i = d, Z_i = z, X_i = x) \right| \leq \|\mathbb{P}_n^W\|_{\mathfrak{P}^+} + \|\mathbb{P}_n^W\|_{\mathfrak{P}^-}$$

$$= O_p^* \left( \sqrt{\frac{\log(n)}{n}} \right). \quad (\text{S37})$$

Then, we have  $\max_{1 \leq j \leq n} |T_{1,j}^\Xi| = O_p^* \left( \sqrt{\log(n)/n} \right)$ . Therefore,  $\sigma_\Xi^2 := \max_{1 \leq j \leq n} \mathbb{E}_{|W_1^n} [\Xi_j^2] = O_p^* \left( \sqrt{\log(n)/n} \right)$ . By the concentration inequality for Gaussian maxima,  $\Pr_{|W_1^n} \left[ \max_{1 \leq j \leq n} |\Xi_j| > C \sqrt{\log(n)} \sigma_\Xi \right] \leq 2n^{-1}$ . It follows that  $\|T_3^\sharp\|_{I_x} = O_p^\sharp \left( \left( \log(n)^3 / (nh^2) \right)^{1/4} \right)$ . It follows from similar arguments and

$$T_4^\sharp(v) \leq \left( \frac{1}{\sqrt{n(2)}} \sum_{j=1}^n h^{-3/2} \left| M' \left( \frac{\hat{\Delta}_j - v}{h} \right) - M' \left( \frac{\Delta_j - v}{h} \right) \right| \right) \left( \max_{1 \leq j \leq n} \left| \frac{1}{\sqrt{n-1}} \sum_{i \neq j} \nu_i q_x(W_j, W_i) \pi_i \right| \right)$$

that  $\|T_4^\sharp\|_{I_x} = O_p^\sharp \left( \log(n) / \sqrt{nh^3} \right)$ . Now we have shown that

$$\frac{1}{\sqrt{n}} \sum_{i=1}^n \nu_i \left\{ \hat{\mathcal{U}}_x^{[1]}(W_i; v) - \tilde{\mathcal{U}}_x^{[1]}(W_i; v) \right\} = O_p^\sharp \left( \sqrt{\frac{\log(n)^3}{nh^3}} + \left( \frac{\log(n)^3}{nh^2} \right)^{1/4} \right), \quad (\text{S38})$$

uniformly in  $v \in I_x$ .

Since  $n^{-1/2} \sum_{i=1}^n \nu_i \sim N(0, 1)$  is independent of the data,  $\Pr_{|W_1^n} \left[ |n^{-1/2} \sum_{i=1}^n \nu_i| > \sqrt{2 \cdot \log(n)} \right] \leq 2n^{-1}$ .  $\hat{\mu}_{\mathcal{U}_x}(v) - \tilde{\mu}_{\mathcal{U}_x}(v)$  can be written as the sum of  $\sqrt{h} \left( \hat{f}_{\Delta X}^{\text{BC}}(v, x) - \tilde{f}_{\Delta X}^{\text{BC}}(v, x) \right)$  and  $-\sqrt{h} n_{(2)}^{-1} \sum_{(j,k)} \mathcal{H}_x^{\text{BC}}(U_j, U_k; v)$ , both of which are  $O_p^* \left( \sqrt{\log(n)/n}, \sqrt{\log(n)/(nh^3)} \right)$ , uniformly in  $v \in I_x$ . It follows from Lemma 5 that

$$\left( \frac{1}{\sqrt{n}} \sum_{i=1}^n \nu_i \right) (\hat{\mu}_{\mathcal{U}_x}(v) - \tilde{\mu}_{\mathcal{U}_x}(v)) = O_p^\sharp \left( \frac{\log(n)}{\sqrt{n}}, n^{-1}, \sqrt{\frac{\log(n)}{nh^3}} \right), \quad (\text{S39})$$

uniformly in  $v \in I_x$ . Decompose

$$\begin{aligned} \frac{1}{\sqrt{n}} \sum_{i=1}^n \nu_i \left\{ \tilde{\mathcal{U}}_x^{[2]}(W_i; v) - \tilde{\mu}_{\mathcal{U}_x}(v) \right\} &= \\ \left( \frac{1}{\sqrt{n}} \sum_{i=1}^n \nu_i \right) \sqrt{h} \left( \frac{1}{n_{(2)}} \sum_{(j,k)} \mathcal{H}_x^{\text{BC}}(U_j, U_k; v) \right) &+ \frac{1}{\sqrt{n}} \sum_{i=1}^n \nu_i \left\{ \frac{1}{n-1} \sum_{j \neq i} h^{-3/2} M' \left( \frac{\Delta_i - v}{h} \right) q_x(W_i, W_j) \pi_j \right\} \\ + \frac{1}{\sqrt{n}} \sum_{i=1}^n \nu_i \left\{ \frac{1}{n} \sum_{j=1}^n h^{-1/2} M \left( \frac{\Delta_j - v}{h} \right) \mathbb{1}(X_j = x) - \frac{1}{n-1} \sum_{j \neq i} h^{-1/2} M \left( \frac{\Delta_j - v}{h} \right) \mathbb{1}(X_j = x) \right\} \\ &=: T_5^\sharp(v) + T_6^\sharp(v) + T_7^\sharp(v). \end{aligned}$$

Similarly,  $\|T_5^\sharp\|_{I_x} = O_p^\sharp \left( \log(n) / \sqrt{n}, n^{-1}, \sqrt{\log(n)/(nh^3)} \right)$ . Write

$$T_6^\sharp(v) = \frac{1}{\sqrt{n}} \sum_{i=1}^n \nu_i h^{-3/2} M' \left( \frac{\Delta_i - v}{h} \right) \mathbb{1}(X_i = x) \left\{ \frac{1}{n-1} \sum_{j \neq i} ((1 - D_i) \mathcal{L}_{1x}(W_j; Y_i) - D_i \mathcal{L}_{0x}(W_j; Y_i)) \right\}.$$

Let  $\mathcal{N}_{dx}(U_i; y) := \mathcal{L}_{dx}(g(D_i, X_i, \epsilon_i), D_i, Z_i, X_i; y)$ . Then, by (S8), (S9), Kosorok (2007, Lemmas 9.6), Kosorok (2007, Lemmas 9.6, 9.8 and 9.9(vi,vii)) and Chernozhukov et al. (2014, Lemma A.6),  $\mathfrak{N} := \{\mathcal{N}_{dx}(\cdot; y) : y \in I_{d'x}\}$  is uniformly VC-type with respect to a constant envelope. By Talagrand's inequality,  $\|\mathbb{G}_n^U\|_{\mathfrak{N}} = O_p^* \left( \sqrt{\log(n)} \right)$

and therefore,  $n^{-1} \sum_{j=1}^n \mathcal{L}_{dx}(W_j; y) = O_p^* \left( \sqrt{\log(n)/n} \right)$ , uniformly in  $y \in I_{d'x}$ . And, therefore, by this result and  $\|\bar{N}_x\|_{I_x} = O_p^*(1)$ , we have  $\sup_{v \in I_x} \mathbb{E}_{|W_1^n} \left[ T_6^\sharp(v)^2 \right] = O_p^* \left( \log(n) / (nh^2) \right)$ . It is easy to see that  $\sup_{v \in I_x} \mathbb{E}_{|W_1^n} \left[ T_7^\sharp(v)^2 \right] = O_p^* \left( n^{-2} \right)$ . Then it follows from arguments used to show  $\|T_1^\sharp\|_{I_x} = O_p^\sharp \left( \log(n) / \sqrt{nh^2} \right)$  that  $\|T_6^\sharp\|_{I_x} = O_p^\sharp \left( \log(n) / \sqrt{nh^2} \right)$  and  $\|T_7^\sharp\|_{I_x} = O_p^\sharp \left( \sqrt{\log(n)/n} \right)$ . Therefore,

$$\frac{1}{\sqrt{n}} \sum_{i=1}^n \nu_i \left\{ \tilde{\mathcal{U}}_x^{[2]}(W_i; v) - \tilde{\mu}_{\mathcal{U}_x}(v) \right\} = O_p^\sharp \left( \frac{\log(n)}{\sqrt{nh^2}}, n^{-1}, \sqrt{\frac{\log(n)}{nh^3}} \right) \quad (\text{S40})$$

uniformly in  $v \in I_x$ .

By (S32), (S39) and (S40), we can write

$$\begin{aligned} S^\sharp(v, x) &= \frac{1}{\sqrt{n}} \sum_{i=1}^n \nu_i \left\{ \tilde{\mathcal{U}}_x^{[1]}(W_i; v) - \tilde{\mu}_{\mathcal{U}_x}(v) \right\} + O_p^\sharp \left( \frac{\log(n)}{\sqrt{nh^2}}, n^{-1}, \sqrt{\frac{\log(n)}{nh^3}} \right) \\ &= T_5^\sharp(v) + T_8^\sharp(v) + T_9^\sharp(v) + O_p^\sharp \left( \frac{\log(n)}{\sqrt{nh^2}}, n^{-1}, \sqrt{\frac{\log(n)}{nh^3}} \right), \end{aligned} \quad (\text{S41})$$

where

$$\begin{aligned} T_8^\sharp(v) &:= \frac{1}{\sqrt{n}} \sum_{i=1}^n \nu_i \left\{ h^{-1/2} M \left( \frac{\Delta_i - v}{h} \right) - \frac{1}{n} \sum_{j=1}^n h^{-1/2} M \left( \frac{\Delta_j - v}{h} \right) \right\} \\ T_9^\sharp(v) &:= \frac{1}{\sqrt{n}} \sum_{i=1}^n \nu_i \left\{ \frac{1}{n-1} \sum_{j \neq i} h^{-3/2} M' \left( \frac{\Delta_j - v}{h} \right) q_x(W_j, W_i) \pi_i \right\}. \end{aligned}$$

We have shown that  $\|T_5^\sharp\|_{I_x} = O_p^\sharp \left( \log(n) / \sqrt{n}, n^{-1}, \sqrt{\log(n) / (nh^3)} \right)$ . Then, by similar arguments used in the proof of Theorem 3, the conditional variances of  $T_8^\sharp(v)$  and  $T_9^\sharp(v)$  satisfy

$$\begin{aligned} \mathbb{E}_{|W_1^n} \left[ T_8^\sharp(v)^2 \right] &= V_{\Delta X}^\dagger(v, x) + O_p^* \left( \sqrt{\frac{\log(n)}{nh}} \right) \\ \mathbb{E}_{|W_1^n} \left[ T_9^\sharp(v)^2 \right] &= V_{\Delta X}^\dagger(v, x) + O_p^* \left( \sqrt{\frac{\log(n)}{nh^3}}, \sqrt{\frac{\log(n)}{nh^3}} \right), \end{aligned}$$

uniformly in  $v \in I_x$ . By similar arguments used in the proof of  $\|T_1^\sharp\|_{I_x} = O_p^\sharp \left( \log(n) / \sqrt{nh^2} \right)$ , we have  $\|T_8^\sharp\|_{I_x} = O_p^\sharp \left( \sqrt{\log(n)} \right)$  and  $\|T_9^\sharp\|_{I_x} = O_p^\sharp \left( \sqrt{\log(n)}, n^{-1}, \sqrt{\log(n) / (nh^3)} \right)$ . Then it follows from (S41) that  $\|S^\sharp(\cdot, x)\|_{I_x} = O_p^\sharp \left( \sqrt{\log(n)}, n^{-1}, \sqrt{\log(n) / (nh^3)} \right)$ . The first conclusion follows from

$$\widehat{S}^\sharp(v|x) - S^\sharp(v|x) = \frac{\widehat{S}^\sharp(v, x)}{p_x} \left( \frac{p_x}{\widehat{p}_x} - 1 \right) + \frac{\widehat{S}^\sharp(v, x) - S^\sharp(v, x)}{p_x}$$

and  $p_x / \widehat{p}_x - 1 = O_p^* \left( \sqrt{\log(n)/n} \right)$ , which follows easily from  $\widehat{p}_x - p_x = O_p^* \left( \sqrt{\log(n)/n} \right)$ .

Write

$$\widehat{Z}^\sharp(v|x) - Z^\sharp(v|x) = \frac{\widehat{S}^\sharp(v, x)}{\sqrt{V_{\Delta X}(v, x)}} \left( \frac{\sqrt{V_{\Delta X}(v, x)}}{\sqrt{\widehat{V}_{\Delta X}(v, x)}} - 1 \right) + \frac{\widehat{S}^\sharp(v, x) - S^\sharp(v, x)}{\sqrt{V_{\Delta X}(v, x)}}. \quad (\text{S42})$$

We have

$$\begin{aligned} \left| \frac{\sqrt{V_{\Delta X}(v, x)}}{\sqrt{\widehat{V}_{\Delta X}(v, x)}} - 1 \right| &\leq \left| \frac{V_{\Delta X}(v, x)}{\widehat{V}_{\Delta X}(v, x)} - 1 \right| \\ &= O_p^* \left( \sqrt{\frac{\log(n)}{nh^2 h_g}} + \frac{h_g^2}{h} + \sqrt{\frac{\log(n)}{nh^4}}, \sqrt{\frac{\log(n)}{nh^4}} \right), \end{aligned} \quad (\text{S43})$$

uniformly in  $v \in I_x$ , where the equality follows from taking  $\gamma = \sqrt{\log(n)/(nh^4)}$  in the deviation bound  $\Pr \left[ \left\| \widehat{V}_{\Delta X}^\dagger(\cdot, x) - V_{\Delta X}^\dagger(\cdot, x) \right\|_{I_x} > C_1 \kappa_1^\dagger \right] \leq C_2 \kappa_2^\dagger$ , which is shown in the proof of Theorem 3. The second conclusion follows from (S42), (S43),  $\|S^\dagger(\cdot, x)\|_{I_x} = O_p^\# \left( \sqrt{\log(n)}, n^{-1}, \sqrt{\log(n)/(nh^3)} \right)$ , Lemma 5 and the first conclusion.  $\blacksquare$

### S3 Proof of Theorem 5

We denote  $\mathbb{P}_n^{W^*} f := n^{-1} \sum_{i=1}^n f(W_i^*)$  and  $\mathbb{G}_n^{W^*} := \sqrt{n}(\mathbb{P}_n^{W^*} - \mathbb{P}_n^W)$ .  $\mathbb{P}_n^{U^*}$  and  $\mathbb{G}_n^{U^*}$  are defined similarly. Let  $\widehat{p}_x^* := n^{-1} \sum_{i=1}^n \mathbb{1}(X_i^* = x)$ ,  $\widehat{f}_{\Delta X}^{\text{BC}*}(v, x) := \widehat{p}_x^* \widehat{f}_{\Delta|X}^*(v|x)$  and let  $\widetilde{f}_{\Delta X}^{\text{BC}*}(v, x)$  be the nonparametric bootstrap analogue of  $\widehat{f}_{\Delta X}^{\text{BC}}(v, x)$ :  $\widetilde{f}_{\Delta X}^{\text{BC}*}(v, x) := (nh)^{-1} \sum_{i=1}^n M((\Delta_i^* - v)/h) \mathbb{1}(X_i^* = x)$ . The following result is a nonparametric bootstrap analogue of Lemma 2. We prove it by adapting the proofs of Lemmas 1 and 2.

**Lemma S1.** *Suppose that the assumptions in the statement of Theorem 5 hold. Then,*

$$\widehat{f}_{\Delta X}^{\text{BC}*}(v, x) - \widetilde{f}_{\Delta X}^{\text{BC}*}(v, x) = \frac{1}{n_{(2)}} \sum_{(i,j)} \mathcal{G}_x^{\text{BC}}(W_i^*, W_j^*; v) + O_p^\# \left( \frac{\log(n)}{nh^2} + \frac{\log(n)^{3/4}}{n^{3/4}h} \right),$$

where the remainder is uniform in  $v \in I_x$ .

**Proof of Lemma S1.** By Talagrand's inequality ( $\mathcal{H} = \mathfrak{D}$ ,  $\sigma = b = F_{\mathfrak{D}} = 1$ ,  $t = \log(n)$ ), we have the deviation bound  $\Pr_{|W_1^n} \left[ \|\mathbb{G}_n^{W^*}\|_{\mathfrak{D}} > C \sqrt{\log(n)} \right] \leq n^{-1}$  and therefore, by Lemma 5,  $\|\widehat{\Pi}_{d'zx}^* - \widehat{\Pi}_{d'zx}\|_{I_{d'x}} = O_p^\# \left( \sqrt{\log(n)/n} \right)$ . Then, by (S1), a nonparametric bootstrap analogue of (S1):

$$\left( \frac{\widehat{\Pi}_{d'0x}^* \left( \widehat{\phi}_{dx}^*(y) \right)}{\widehat{p}_{0x}^*} - \frac{\widehat{\Pi}_{d'1x}^* \left( \widehat{\phi}_{dx}^*(y) \right)}{\widehat{p}_{1x}^*} \right) + \left( \frac{\widehat{\Pi}_{d'0x}^* (y)}{\widehat{p}_{0x}^*} - \frac{\widehat{\Pi}_{d'1x}^* (y)}{\widehat{p}_{1x}^*} \right) = \varepsilon_n^*,$$

where  $|\varepsilon_n^*| \leq 1$ , and by Lemma 5, we have  $\|\widehat{\phi}_{dx}^* - \widehat{\phi}_{dx}\|_{I_{d'x}} = O_p^\# \left( \sqrt{\log(n)/n} \right)$  and also  $\|\widehat{\phi}_{dx}^* - \phi_{dx}\|_{I_{d'x}} = O_p^\# \left( \sqrt{\log(n)/n} \right)$ .

Then we can easily show a bootstrap analogue of (S5). Then, similarly, we decompose  $\widehat{\Pi}_{d'zx}^* \left( \widehat{\phi}_{dx}^*(y) \right) - \widehat{\Pi}_{d'zx} \left( \widehat{\phi}_{dx}(y) \right)$  into the sum of  $\widehat{\Pi}_{d'zx}^* \left( \widehat{\phi}_{dx}^*(y) \right) - \widehat{\Pi}_{d'zx} \left( \widehat{\phi}_{dx}^*(y) \right)$  and  $\widehat{\Pi}_{d'zx} \left( \widehat{\phi}_{dx}^*(y) \right) - \widehat{\Pi}_{d'zx} \left( \widehat{\phi}_{dx}(y) \right)$ . Next, we show that

$$\begin{aligned} \widehat{\Pi}_{d'zx}^* \left( \widehat{\phi}_{dx}^*(y) \right) - \widehat{\Pi}_{d'zx} \left( \widehat{\phi}_{dx}^*(y) \right) &= \widehat{\Pi}_{d'zx}^* (\phi_{dx}(y)) - \widehat{\Pi}_{d'zx} (\phi_{dx}(y)) + O_p^\# \left( \left( \frac{\log(n)}{n} \right)^{3/4} \right) \\ \widehat{\Pi}_{d'zx} \left( \widehat{\phi}_{dx}^*(y) \right) - \widehat{\Pi}_{d'zx} \left( \widehat{\phi}_{dx}(y) \right) &= \Pi_{d'zx} \left( \widehat{\phi}_{dx}^*(y) \right) - \Pi_{d'zx} \left( \widehat{\phi}_{dx}(y) \right) + O_p^\# \left( \left( \frac{\log(n)}{n} \right)^{3/4} \right), \end{aligned} \quad (\text{S44})$$

uniformly in  $y \in I_{d'x}$ . Denote  $\hat{\Lambda}_{d'zx}^*(y, y') := \hat{\Pi}_{d'zx}^*(y) - \hat{\Pi}_{d'zx}^*(y')$ . Let  $\hat{\sigma}_{\mathfrak{P}^+}^2 := \sup_{f \in \mathfrak{P}^+} \mathbb{P}_n^W f^2$ . Then,  $\hat{\sigma}_{\mathfrak{P}^+}^2 \leq \sigma_{\mathfrak{P}^+}^2 + \|\mathbb{P}_n^W - \mathbb{P}^W\|_{\mathfrak{P}^+} = O_p^*\left(\sqrt{\log(n)/n}\right)$ . By Talagrand's inequality ( $\mathcal{H} = \mathfrak{P}^+$ ,  $b = F_{\mathfrak{P}^+} = 1$ ,  $\sigma = \hat{\sigma}_{\mathfrak{P}^+} \vee n^{-1/4}b$ ,  $t = \log(n)$ ),  $\Pr_{|W_1^n} \left[ \|\mathbb{G}_n^{W*}\|_{\mathfrak{P}^+} > C(\hat{\sigma}_{\mathfrak{P}^+} \vee n^{-1/4}) \sqrt{\log(n)} \right] \leq n^{-1}$ . Similarly, we define  $\hat{\sigma}_{\mathfrak{P}^-}^2$  and have a deviation bound  $\Pr_{|W_1^n} \left[ \|\mathbb{G}_n^{W*}\|_{\mathfrak{P}^-} > C(\hat{\sigma}_{\mathfrak{P}^-} \vee n^{-1/4}) \sqrt{\log(n)} \right] \leq n^{-1}$ . With probability greater than  $1 - C_3 n^{-1}$ ,  $\Pr_{|W_1^n} \left[ \left\| \hat{\phi}_{dx}^* - \phi_{dx} \right\|_{I_{d'x}} > C_1 \sqrt{\log(n)/n} \right] > C_2 n^{-1}$ . Then the first result in (S44) follows from Lemma 5,  $\hat{\sigma}_{\mathfrak{P}^+} = O_p^*\left((\log(n)/n)^{1/4}\right)$ ,  $\hat{\sigma}_{\mathfrak{P}^-} = O_p^*\left((\log(n)/n)^{1/4}\right)$  and

$$\begin{aligned} & \Pr_{|W_1^n} \left[ \sup_{y \in I_{d'x}} \left| \hat{\Lambda}_{d'zx}^* \left( \hat{\phi}_{dx}^*(y), \phi_{dx}(y) \right) - \hat{\Lambda}_{d'zx} \left( \hat{\phi}_{dx}^*(y), \phi_{dx}(y) \right) \right| > C \left( \hat{\sigma}_{\mathfrak{P}^+} \vee n^{-1/4} + \hat{\sigma}_{\mathfrak{P}^-} \vee n^{-1/4} \right) \sqrt{\frac{\log(n)}{n}} \right] \\ & \leq \Pr_{|W_1^n} \left[ \left\| \mathbb{G}_n^{W*} \right\|_{\mathfrak{P}^+} > C \left( \hat{\sigma}_{\mathfrak{P}^+} \vee n^{-1/4} \right) \sqrt{\log(n)} \right] + \Pr_{|W_1^n} \left[ \left\| \mathbb{G}_n^{W*} \right\|_{\mathfrak{P}^-} > C \left( \hat{\sigma}_{\mathfrak{P}^-} \vee n^{-1/4} \right) \sqrt{\log(n)} \right] \\ & \quad + \Pr_{|W_1^n} \left[ \left\| \hat{\phi}_{dx}^* - \phi_{dx} \right\|_{I_{d'x}} > C_1 \sqrt{\frac{\log(n)}{n}} \right] = O_p^*(n^{-1}). \end{aligned}$$

Similarly, the second result in (S44) follows from Lemma 5,  $\sigma_{\mathfrak{P}^+} = O\left((\log(n)/n)^{1/4}\right)$ ,  $\sigma_{\mathfrak{P}^-} = O\left((\log(n)/n)^{1/4}\right)$  and

$$\begin{aligned} & \Pr_{|W_1^n} \left[ \sup_{y \in I_{d'x}} \left| \hat{\Lambda}_{d'zx} \left( \hat{\phi}_{dx}^*(y), \hat{\phi}_{dx}(y) \right) - \Lambda_{d'zx} \left( \hat{\phi}_{dx}^*(y), \hat{\phi}_{dx}(y) \right) \right| > C \left( \sigma_{\mathfrak{P}^+} \vee n^{-1/4} + \sigma_{\mathfrak{P}^-} \vee n^{-1/4} \right) \sqrt{\frac{\log(n)}{n}} \right] \\ & \leq \Pr_{|W_1^n} \left[ \left\| \mathbb{G}_n^W \right\|_{\mathfrak{P}^+} > C \left( \sigma_{\mathfrak{P}^+} \vee n^{-1/4} \right) \sqrt{\frac{\log(n)}{n}} \right] + \Pr_{|W_1^n} \left[ \left\| \mathbb{G}_n^W \right\|_{\mathfrak{P}^-} > C \left( \sigma_{\mathfrak{P}^-} \vee n^{-1/4} \right) \sqrt{\frac{\log(n)}{n}} \right] \\ & \quad + \Pr_{|W_1^n} \left[ \left\| \hat{\phi}_{dx}^* - \hat{\phi}_{dx} \right\|_{I_{d'x}} > C_1 \sqrt{\frac{\log(n)}{n}} \right] = O_p^*(n^{-1}). \end{aligned}$$

Then, by using (S44), a bootstrap analogue of (S5) and tedious algebra, we have  $\hat{\phi}_{dx}^*(y) - \hat{\phi}_{dx}(y) = n^{-1} \sum_{i=1}^n \mathcal{L}_{dx}(W_i^*; y) - n^{-1} \sum_{i=1}^n \mathcal{L}_{dx}(W_i; y) + O_p^\# \left( (\log(n)/n)^{3/4} \right)$  and by Lemmas 1 and 5, a linear representation in the bootstrap world holds:

$$\hat{\phi}_{dx}^*(y) - \phi_{dx}(y) = \frac{1}{n} \sum_{i=1}^n \mathcal{L}_{dx}(W_i^*; y) + O_p^\# \left( \left( \frac{\log(n)}{n} \right)^{3/4} \right), \quad (\text{S45})$$

uniformly in  $y \in I_{d'x}$ . Let  $\hat{\sigma}_{\mathfrak{J}}^2 := \sup_{f \in \mathfrak{J}} \mathbb{P}_n^U f^2$ . Then we have  $\hat{\sigma}_{\mathfrak{J}}^2 \leq h^{-1} (\|\mathbb{P}^U\|_{\mathfrak{J}} + \|\mathbb{P}_n^U - \mathbb{P}^U\|_{\mathfrak{J}}) = O_p^*(h^{-1})$ . By Talagrand's inequality ( $\mathcal{H} = \mathfrak{J}$ ,  $b = F_{\mathfrak{J}} = h^{-1}$ ,  $\sigma = \hat{\sigma}_{\mathfrak{J}} \vee n^{-1/2}b$ ,  $t = \log(n)$ ), we have

$$\Pr_{|W_1^n} \left[ \left\| \mathbb{G}_n^{U*} \right\|_{\mathfrak{J}} > C \left( \hat{\sigma}_{\mathfrak{J}} \vee (nh^2)^{-1/2} \right) \sqrt{\log(n)} \right] \leq n^{-1}.$$

By Lemma 5,  $\|\mathbb{G}_n^{U*}\|_{\mathfrak{J}} = O_p^\# \left( \sqrt{\log(n)/h} \right)$ . Then,  $\|\mathbb{P}_n^{U*}\|_{\mathfrak{J}} \leq \|\mathbb{P}_n^{U*} - \mathbb{P}_n^U\|_{\mathfrak{J}} + \|\mathbb{P}_n^U - \mathbb{P}^U\|_{\mathfrak{J}} + \|\mathbb{P}^U\|_{\mathfrak{J}} = O_p^\#(1)$ . Then, by these results, a bootstrap analogue of (S12) (i.e.,  $\max_{1 \leq i \leq n} \left| \hat{\Delta}_i^* - \Delta_i^* \right| \mathbb{1}(X_i^* = x) = O_p^\# \left( \sqrt{\log(n)/n} \right)$ ) which follows from  $\left\| \hat{\phi}_{dx}^* - \phi_{dx} \right\|_{I_{d'x}} = O_p^\# \left( \sqrt{\log(n)/n} \right)$  and Taylor expansion, we have

$$\widehat{f}_{\Delta X}^{\text{BC}*}(v, x) - \widetilde{f}_{\Delta X}^{\text{BC}*}(v, x) = \frac{1}{n} \sum_{i=1}^n \frac{1}{h^2} M' \left( \frac{\Delta_i^* - v}{h} \right) \left( \hat{\Delta}_i^* - \Delta_i^* \right) \mathbb{1}(X_i^* = x) + O_p^\# \left( \frac{\log(n)}{nh^2} \right).$$

Then the conclusion follows from this result, (S45) and  $\|\mathbb{P}_n^{U^*}\|_{\mathcal{J}} = O_p^\sharp(1)$ . ■

**Lemma S2.** *Suppose that the assumptions in the statement of Theorem 5 hold. Then,*

$$\begin{aligned} \widehat{f}_{\Delta X}^{\text{BC}*}(v, x) - \widehat{f}_{\Delta X}^{\text{BC}*}(v, x) &= \frac{1}{n^2} \sum_{i=1}^n \sum_{j=1}^n \mathcal{H}_x^{\text{BC}}(U_i, U_j; v) + \left\{ \frac{1}{n} \sum_{i=1}^n \mathcal{H}_x^{\text{BC}[1]}(U_i^*; v) - \frac{1}{n} \sum_{i=1}^n \mathcal{H}_x^{\text{BC}[1]}(U_i; v) \right\} \\ &\quad + O_p^\sharp \left( \left( \frac{\log(n)}{n^3 h^5} \right)^{1/4}, \left( \frac{\log(n)}{n h^3} \right)^{1/4}, \sqrt{\frac{\log(n)}{n h^3}} \right), \end{aligned}$$

where the remainder is uniform in  $v \in I_x$ .

**Proof of Lemma S2.** It is easy to check that

$$\mathcal{G}_x^{\text{BC}}(W_i^*, W_j^*; v) = \mathcal{G}_x^{\text{BC}}((g(D_i^*, X_i^*, \epsilon_i^*), D_i^*, Z_i^*, X_i^*), (g(D_j^*, X_j^*, \epsilon_j^*), D_j^*, Z_j^*, X_j^*); v) = \mathcal{H}_x^{\text{BC}}(U_i^*, U_j^*; v).$$

Denote

$$\begin{aligned} \overline{\mathcal{H}}_x^{[1]}(u; v) &:= \mathbb{E}_{|W_1^n} [\mathcal{H}_x^{\text{BC}}(U^*, u; v)] = \frac{1}{n} \sum_{j=1}^n \mathcal{H}_x^{\text{BC}}(U_j, u; v) \\ \overline{\mathcal{H}}_x^{[2]}(u; v) &:= \mathbb{E}_{|W_1^n} [\mathcal{H}_x^{\text{BC}}(u, U^*; v)] = \frac{1}{n} \sum_{j=1}^n \mathcal{H}_x^{\text{BC}}(u, U_j; v) \\ \overline{\mu}_{\mathcal{H}_x^{\text{BC}}}(v) &:= \mathbb{E}_{|W_1^n} [\mathcal{H}_x^{\text{BC}}(U_1^*, U_2^*; v)] = \frac{1}{n^2} \sum_{i=1}^n \sum_{j=1}^n \mathcal{H}_x^{\text{BC}}(U_i, U_j; v). \end{aligned}$$

Then, by Hoeffding decomposition,

$$\begin{aligned} \frac{1}{n_{(2)}} \sum_{(i,j)} \mathcal{H}_x^{\text{BC}}(U_i^*, U_j^*; v) &= \overline{\mu}_{\mathcal{H}_x^{\text{BC}}}(v) + \left\{ \frac{1}{n} \sum_{i=1}^n \overline{\mathcal{H}}_x^{[1]}(U_i^*; v) - \overline{\mu}_{\mathcal{H}_x^{\text{BC}}}(v) \right\} + \left\{ \frac{1}{n} \sum_{i=1}^n \overline{\mathcal{H}}_x^{[2]}(U_i^*; v) - \overline{\mu}_{\mathcal{H}_x^{\text{BC}}}(v) \right\} \\ &\quad + \frac{1}{n_{(2)}} \sum_{(i,j)} \left\{ \mathcal{H}_x^{\text{BC}}(U_i^*, U_j^*; v) - \overline{\mathcal{H}}_x^{[1]}(U_i^*; v) - \overline{\mathcal{H}}_x^{[2]}(U_j^*; v) + \overline{\mu}_{\mathcal{H}_x^{\text{BC}}}(v) \right\}. \quad (\text{S46}) \end{aligned}$$

Denote

$$\begin{aligned} T_1^*(v) &:= \frac{1}{n} \sum_{i=1}^n \left( \overline{\mathcal{H}}_x^{[1]}(U_i^*; v) - \mathcal{H}_x^{\text{BC}[1]}(U_i^*; v) \right) - \left( \overline{\mu}_{\mathcal{H}_x^{\text{BC}}}(v) - \frac{1}{n} \sum_{i=1}^n \mathcal{H}_x^{\text{BC}[1]}(U_i; v) \right) \\ T_2^*(v) &:= \frac{1}{n} \sum_{i=1}^n \overline{\mathcal{H}}_x^{[2]}(U_i^*; v) - \overline{\mu}_{\mathcal{H}_x^{\text{BC}}}(v) \\ T_3^*(v) &:= \frac{1}{n_{(2)}} \sum_{(i,j)} \left\{ \mathcal{H}_x^{\text{BC}}(U_i^*, U_j^*; v) - \overline{\mathcal{H}}_x^{[1]}(U_i^*; v) - \overline{\mathcal{H}}_x^{[2]}(U_j^*; v) + \overline{\mu}_{\mathcal{H}_x^{\text{BC}}}(v) \right\}. \end{aligned}$$

Then, by (S46),

$$\frac{1}{n_{(2)}} \sum_{(i,j)} \mathcal{H}_x^{\text{BC}}(U_i^*, U_j^*; v) = \overline{\mu}_{\mathcal{H}_x^{\text{BC}}}(v) + \frac{1}{n} \sum_{i=1}^n \mathcal{H}_x^{\text{BC}[1]}(U_i^*; v) - \frac{1}{n} \sum_{i=1}^n \mathcal{H}_x^{\text{BC}[1]}(U_i; v) + T_1^*(v) + T_2^*(v) + T_3^*(v).$$

Note that  $E_{|W_1^n} \left[ \left( \overline{\mathcal{H}}_x^{[1]}(U^*; v) - \mathcal{H}_x^{\text{BC}[1]}(U^*; v) \right)^2 \right]$  can be represented by a V-statistic:

$$\begin{aligned} E_{|W_1^n} \left[ \left( \overline{\mathcal{H}}_x^{[1]}(U^*; v) - \mathcal{H}_x^{\text{BC}[1]}(U^*; v) \right)^2 \right] &= \\ \frac{1}{n^3} \sum_{i=1}^n \sum_{j=1}^n \sum_{k=1}^n &\left( \mathcal{H}_x^{\text{BC}}(U_j, U_i; v) - \mathcal{H}_x^{\text{BC}[1]}(U_i; v) \right) \left( \mathcal{H}_x^{\text{BC}}(U_k, U_i; v) - \mathcal{H}_x^{\text{BC}[1]}(U_i; v) \right) \\ &=: \frac{1}{n^3} \sum_{i=1}^n \sum_{j=1}^n \sum_{k=1}^n \mathcal{V}_x(U_i, U_j, U_k; v). \end{aligned} \quad (\text{S47})$$

It is easy to check that

$$\frac{1}{n^3} \sum_{i=1}^n \sum_{j=1}^n \sum_{k=1}^n \mathcal{V}_x(U_i, U_j, U_k; v) - \frac{1}{n_{(3)}} \sum_{(i,j,k)} \mathcal{V}_x(U_i, U_j, U_k; v) = O\left((nh^4)^{-1}\right), \quad (\text{S48})$$

uniformly in  $v \in I_x$ , and the kernel of the U-statistic  $n_{(3)}^{-1} \sum_{(i,j,k)} \mathcal{V}_x(U_i, U_j, U_k; v)$  is degenerate of order one (see, e.g., Definition 5.1 of CK). Since both of  $\mathfrak{H}^{\text{BC}} := \{\mathcal{H}_x^{\text{BC}}(\cdot; v) : v \in I_x\}$  and  $\mathfrak{H}^{\text{BC}[1]} := \{\mathcal{H}_x^{\text{BC}[1]}(\cdot; v) : v \in I_x\}$  are uniformly VC-type with respect to a constant envelope that is a multiple of  $h^{-2}$ , by Chernozhukov et al. (2014, Lemma A.6),  $\mathfrak{V} := \{\mathcal{V}_x(\cdot; v) : v \in I_x\}$  is uniformly VC-type with respect to a constant envelope  $F_{\mathfrak{V}} \propto h^{-4}$ . By Hoeffding decomposition of the U-process  $\{\mathbb{U}_n^{(3)} f : f \in \mathfrak{V}\}$  and using the maximal inequality of CK Corollary 5.6,  $E \left[ \left\| \mathbb{U}_n^{(3)} \right\|_{\mathfrak{V}} \right] = O(n^{-1/2} h^{-4})$ . Denote  $\mathfrak{R} := \{\overline{\mathcal{H}}_x^{[1]}(\cdot; v) - \mathcal{H}_x^{\text{BC}[1]}(\cdot; v) : v \in I_x\}$  and

$$\widehat{\sigma}_{\mathfrak{R}}^2 := \sup_{f \in \mathfrak{R}} \mathbb{P}_n^U f^2 = \sup_{v \in I_x} E_{|W_1^n} \left[ \left( \overline{\mathcal{H}}_x^{[1]}(U^*; v) - \mathcal{H}_x^{\text{BC}[1]}(U^*; v) \right)^2 \right].$$

Then, by (S47) and (S48),  $E \left[ \widehat{\sigma}_{\mathfrak{R}}^2 \right] = n^{-1/2} E \left[ \left\| \mathbb{U}_n^{(3)} \right\|_{\mathfrak{V}} \right] = O\left((nh^4)^{-1}\right)$ . By Markov's inequality,

$$\Pr \left[ \widehat{\sigma}_{\mathfrak{R}} > (E \left[ \widehat{\sigma}_{\mathfrak{R}}^2 \right] / (\log(n) h))^{1/4} \right] \leq \sqrt{\log(n) h \cdot E \left[ \widehat{\sigma}_{\mathfrak{R}}^2 \right]}$$

and, therefore,  $\widehat{\sigma}_{\mathfrak{R}} = O_p \left( (\log(n))^{-1/4} (nh^5)^{-1/4}, \sqrt{\log(n) / (nh^3)} \right)$ . By CK Lemma 5.4, the (data-dependent) function class  $\overline{\mathfrak{H}}^{[1]} := \{\overline{\mathcal{H}}_x^{[1]}(\cdot; v) : v \in I_x\}$  is uniformly VC-type (conditionally on the data) with respect to a constant envelope  $F_{\overline{\mathfrak{H}}^{[1]}} = F_{\mathfrak{H}^{\text{BC}}} \propto h^{-2}$ , i.e., (37) (with  $\mathfrak{F}_n = \overline{\mathfrak{H}}^{[1]}$  and  $F_{\mathfrak{F}_n} = F_{\overline{\mathfrak{H}}^{[1]}}$ ) is satisfied with VC characteristics that do not depend on the data. Then, by Chernozhukov et al. (2014, Lemma A.6),  $\mathfrak{R}$  is also uniformly VC-type (conditionally on the data) with respect to the constant envelope  $F_{\mathfrak{R}} = 2F_{\mathfrak{H}^{\text{BC}}} \propto h^{-2}$ . Then, by Talagrand's inequality ( $\mathcal{F} = \mathfrak{R}$ ,  $b = F_{\mathfrak{R}}$ ,  $\sigma = \widehat{\sigma}_{\mathfrak{R}} \vee n^{-1/2} b$ ,  $t = \log(n)$ ), Lemma 5 and the fact  $\|T_1^*\|_{I_x} = n^{-1/2} \|\mathbb{G}_n^{U^*}\|_{\mathfrak{R}}, \|T_1^*\|_{I_x} = O_p^\# \left( (\log(n) / (n^3 h^5))^{1/4}, n^{-1}, \sqrt{\log(n) / (nh^3)} \right)$ .

Denote  $\overline{H}_x(e) := n^{-1} \sum_{i=1}^n \{ \mathbb{1}(\epsilon_i \leq e) - F_{\epsilon|X}(e|x) \} \pi_i$ . By Talagrand's inequality, we can easily show that  $\|\overline{H}_x\|_{[\underline{\epsilon}_x, \bar{\epsilon}_x]} = O_p^* \left( \sqrt{\log(n)/n} \right)$ . Then,  $\overline{\mathcal{H}}_x^{[2]}(U_i^*; v) = h^{-2} M'((\Delta_x(\epsilon_i^*) - v)/h) \varpi_x(U_i^*) \overline{H}_x(\epsilon_i^*)$ . It can be easily verified by using arguments in the proof of Lemma 3 that the (data-dependent) function class  $\overline{\mathfrak{H}}^{[2]} := \{\overline{\mathcal{H}}_x^{[2]}(\cdot; v) : v \in I_x\}$  is uniformly VC-type (conditionally on the data) with respect to a constant envelope that is a multiple of  $h^{-2} \|\overline{H}_x\|_{[\underline{\epsilon}_x, \bar{\epsilon}_x]}$ , with VC characteristics that do not depend on the data. Then, by CK Corollary

5.6,  $E_{|W_1^n} \left[ \left\| \mathbb{G}_n^{U^*} \right\|_{\bar{\mathcal{Y}}^{[2]}} \right] = O_p^* \left( \sqrt{\log(n) / (nh^4)} \right)$ . Then, by Markov's inequality,

$$\Pr_{|W_1^n} \left[ \left\| \mathbb{G}_n^{U^*} \right\|_{\bar{\mathcal{Y}}^{[2]}} > h^{-1/4} \sqrt{E_{|W_1^n} \left[ \left\| \mathbb{G}_n^{U^*} \right\|_{\bar{\mathcal{Y}}^{[2]}} \right]} \right] \leq h^{1/4} \sqrt{E_{|W_1^n} \left[ \left\| \mathbb{G}_n^{U^*} \right\|_{\bar{\mathcal{Y}}^{[2]}} \right]} = O_p^* \left( \left( \frac{\log(n)}{nh^3} \right)^{1/4} \right).$$

By Lemma 5 and  $\|T_2^*\|_{I_x} = n^{-1/2} \|\mathbb{G}_n^{U^*}\|_{\bar{\mathcal{Y}}^{[2]}}$ ,  $\|T_2^*\|_{I_x} = O_p^\# \left( (\log(n) / (n^3 h^5))^{1/4}, (\log(n) / (nh^3))^{1/4}, n^{-1} \right)$ .

It is easy to check that by CK Corollary 5.6,  $E_{|W_1^n} [\|T_3^*\|_{I_x}] = O_p^* \left( (nh^2)^{-1} \right)$ . Then, by Markov's inequality,

$$\Pr_{|W_1^n} \left[ \|T_3^*\|_{I_x} > \frac{\sqrt{E_{|W_1^n} [\|T_3^*\|_{I_x}]}}{(nh)^{1/4}} \right] \leq (nh)^{1/4} \sqrt{E_{|W_1^n} [\|T_3^*\|_{I_x}]} = O_p^* \left( (nh^3)^{-1/4} \right)$$

Therefore, by Lemma 5, we have  $\|T_3^*\|_{I_x} = O_p^\# \left( (n^3 h^5)^{-1/4}, (nh^3)^{-1/4}, n^{-1} \right)$ . ■

**Lemma S3.** Suppose that the assumptions in the statement of Theorem 5 hold. Then,

$$\begin{aligned} S^*(v|x) &= \frac{1}{\sqrt{n}} \sum_{i=1}^n \left( \mathcal{M}_x^{[1]}(U_i^*; v) - \frac{1}{n} \sum_{i=1}^n \mathcal{M}_x^{[1]}(U_i; v) \right) \\ &\quad + O_p^\# \left( \left( \frac{\log(n)}{nh^3} \right)^{1/4} + \sqrt{\log(n)h}, \left( \frac{\log(n)}{nh^3} \right)^{1/4}, \sqrt{\frac{\log(n)}{nh^3}} \right) \\ Z^*(v|x) &= \frac{1}{\sqrt{n}} \sum_{i=1}^n \left( \frac{\mathcal{M}_x^{[1]}(U_i^*; v)}{\sqrt{V_{\Delta|X}(v|x)}} - \frac{1}{n} \sum_{i=1}^n \frac{\mathcal{M}_x^{[1]}(U_i; v)}{\sqrt{V_{\Delta|X}(v|x)}} \right) \\ &\quad + O_p^\# \left( \left( \frac{\log(n)}{nh^3} \right)^{1/4} + \sqrt{\log(n)h} + \frac{\log(n)}{\sqrt{nh^2 h_g}} + \frac{\sqrt{\log(n)h_g^2}}{h} + \frac{\log(n)}{\sqrt{nh^4}}, \left( \frac{\log(n)}{nh^3} \right)^{1/4}, \sqrt{\frac{\log(n)}{nh^4}} \right) \end{aligned}$$

uniformly in  $v \in I_x$ .

**Proof of Lemma S3.** It can be easily verified that the difference between  $n^{-2} \sum_{i=1}^n \sum_{j=1}^n \mathcal{H}_x^{\text{BC}}(U_i, U_j; v)$  and  $n_{(2)}^{-1} \sum_{(i,j)} \mathcal{H}_x^{\text{BC}}(U_i, U_j; v)$  is  $O \left( (nh^2)^{-1} \right)$ , uniformly in  $v \in I_x$ . We decompose  $\hat{f}_{\Delta X}^{\text{BC}*}(v, x) - \hat{f}_{\Delta X}^{\text{BC}}(v, x)$  into the sum of  $\hat{f}_{\Delta X}^{\text{BC}*}(v, x) - \tilde{f}_{\Delta X}^{\text{BC}*}(v, x)$ ,  $\tilde{f}_{\Delta X}^{\text{BC}*}(v, x) - \tilde{f}_{\Delta X}^{\text{BC}}(v, x)$  and  $\tilde{f}_{\Delta X}^{\text{BC}}(v, x) - \hat{f}_{\Delta X}^{\text{BC}}(v, x)$ . Then, by Lemmas 2, 5 and S2,

$$\begin{aligned} \hat{f}_{\Delta X}^{\text{BC}*}(v, x) - \hat{f}_{\Delta X}^{\text{BC}}(v, x) &= \left\{ \frac{1}{n} \sum_{i=1}^n \mathcal{H}_x^{\text{BC}[1]}(U_i^*; v) - \frac{1}{n} \sum_{i=1}^n \mathcal{H}_x^{\text{BC}[1]}(U_i; v) \right\} + \left\{ \hat{f}_{\Delta X}^{\text{BC}*}(v, x) - \tilde{f}_{\Delta X}^{\text{BC}}(v, x) \right\} \\ &\quad + O_p^\# \left( \left( \frac{\log(n)}{n^3 h^5} \right)^{1/4}, \left( \frac{\log(n)}{nh^3} \right)^{1/4}, \sqrt{\frac{\log(n)}{nh^3}} \right), \quad (\text{S49}) \end{aligned}$$

uniformly in  $v \in I_x$ . Then, let  $\hat{\sigma}_{\mathfrak{H}^{\text{BC}[1]}}^2 := \sup_{f \in \mathfrak{H}^{\text{BC}[1]}} \mathbb{P}_n^U f^2$  and  $\check{\mathfrak{H}}^{[1]} := \left\{ \mathcal{H}_x^{\text{BC}[1]}(\cdot; v)^2 : v \in I_x \right\}$ . By Chernozhukov et al. (2014, Lemma A.6),  $\check{\mathfrak{H}}^{[1]}$  is uniformly VC-type with respect to a constant envelope  $F_{\check{\mathfrak{H}}^{[1]}} \propto h^{-4}$ . Then,  $\hat{\sigma}_{\mathfrak{H}^{\text{BC}[1]}}^2 \leq \sigma_{\mathfrak{H}^{\text{BC}[1]}}^2 + \|\mathbb{P}_n^U - \mathbb{P}^U\|_{\check{\mathfrak{H}}^{[1]}}$ . It was shown in the proof of Lemma 3 that  $\sigma_{\mathfrak{H}^{\text{BC}[1]}}^2 = O(h^{-1})$ . Let  $\sigma_{\check{\mathfrak{H}}^{[1]}}^2 := \sup_{f \in \check{\mathfrak{H}}^{[1]}} \mathbb{P}^U f^2$ . It is easy to check that by change of variables,  $\sigma_{\check{\mathfrak{H}}^{[1]}}^2 = O(h^{-4})$  and therefore, by Talagrand's inequality ( $\mathcal{F} = \check{\mathfrak{H}}^{[1]}$ ,  $b = F_{\check{\mathfrak{H}}^{[1]}}$ ,  $\sigma = \sigma_{\check{\mathfrak{H}}^{[1]}} \vee n^{-1/2}b$ ,  $t = \log(n)$ ),  $\|\mathbb{G}_n^U\|_{\check{\mathfrak{H}}^{[1]}} = O_p^* \left( \sqrt{\log(n)/h^4} + \log(n)/(n^{1/2}h^4) \right)$  and therefore,  $\hat{\sigma}_{\mathfrak{H}^{\text{BC}[1]}}^2 = O_p^*(h^{-1})$ . By using Talagrand's inequality again ( $\mathcal{F} = \mathfrak{H}^{\text{BC}[1]}$ ,  $b = F_{\mathfrak{H}^{\text{BC}[1]}}$ ,  $\sigma =$

$\hat{\sigma}_{\mathfrak{S}^{\text{bc}[1]}} \vee n^{-1/2}b$ ,  $t = \log(n)$ ) and Lemma 5,  $\|\mathbb{G}_n^{U*}\|_{\mathfrak{S}^{\text{bc}[1]}} = O_p^\# \left( \sqrt{\log(n)/h} \right)$  and therefore, the first term on the right hand side of (S49) is  $O_p^\# \left( \sqrt{\log(n)/nh} \right)$ , uniformly in  $v \in I_x$ . Similarly, by Talagrand's inequality,  $\left\| \tilde{f}_{\Delta X}^{\text{BC}*}(\cdot, x) - \tilde{f}_{\Delta X}^{\text{BC}}(\cdot, x) \right\|_{I_x} = O_p^\# \left( \sqrt{\log(n)/(nh)} \right)$ . Therefore,

$$\left\| \hat{f}_{\Delta X}^{\text{BC}*}(\cdot, x) - \hat{f}_{\Delta X}^{\text{BC}}(\cdot, x) \right\|_{I_x} = O_p^\# \left( \sqrt{\frac{\log(n)}{nh}}, \left( \frac{\log(n)}{nh^3} \right)^{1/4}, \sqrt{\frac{\log(n)}{nh^3}} \right). \quad (\text{S50})$$

By Lemma 5 and Hoeffding's inequality, we have  $\hat{p}_x^* - \hat{p}_x = O_p^\# \left( \sqrt{\log(n)/n} \right)$ . And, by using  $\hat{p}_x - p_x = O_p^\# \left( \sqrt{\log(n)/n} \right)$ , Lemma 5, (S49), (S50) and

$$\begin{aligned} S^*(v|x) &= \frac{1}{p_x} \sqrt{nh} \left( \hat{f}_{\Delta X}^{\text{BC}*}(v, x) - \hat{f}_{\Delta X}^{\text{BC}}(v, x) \right) + \left( \frac{1}{\hat{p}_x} - \frac{1}{p_x} \right) \sqrt{nh} \left( \hat{f}_{\Delta X}^{\text{BC}*}(v, x) - \hat{f}_{\Delta X}^{\text{BC}}(v, x) \right) \\ &\quad + \frac{\sqrt{nh} \hat{f}_{\Delta X}^{\text{BC}*}(v, x)}{\hat{p}_x} \left( \frac{\hat{p}_x}{\hat{p}_x^*} - 1 \right), \end{aligned}$$

we have the first conclusion.

It is easy to see that  $\|S^*(\cdot|x)\|_{I_x} = O_p^\# \left( \sqrt{\log(n)}, (\log(n)/(nh^3))^{1/4}, \sqrt{\log(n)/(nh^3)} \right)$ . Then the second conclusion follows from this result, the first conclusion and similar arguments used in the proof of the second part of Lemma 6.  $\blacksquare$

**Proof of Theorem 5.** By Lemma S3,

$$\|S^*(\cdot|x)\|_{I_x} - \|\mathbb{G}_n^{U*}\|_{\mathfrak{M}^{[1]}} = O_p^\# \left( \left( \frac{\log(n)}{nh^3} \right)^{1/4} + \sqrt{\log(n)h}, \left( \frac{\log(n)}{nh^3} \right)^{1/4}, \sqrt{\frac{\log(n)}{nh^3}} \right). \quad (\text{S51})$$

We apply Chernozhukov et al. (2016, Theorem 2.3) with  $\mathcal{F} = \mathfrak{M}_\pm^{[1]}$ ,  $B = 0$ ,  $\sigma = \bar{\sigma}_{\mathfrak{M}^{[1]}}$ ,  $b = F_{\mathfrak{M}^{[1]}}$  and  $q = \infty$ . For any fixed coupling error  $\gamma \in (0, 1)$ , there exists a random variable  $\tilde{Z}_{\mathfrak{M}_\pm^{[1]}, \gamma}^*$  such that (1)  $\tilde{Z}_{\mathfrak{M}_\pm^{[1]}, \gamma}^*$  is independent of the data; (2)  $\tilde{Z}_{\mathfrak{M}_\pm^{[1]}, \gamma}^*$  has the same distribution as  $\|\mathbb{G}_n^U\|_{\mathfrak{M}^{[1]}}$ ; (3)  $\tilde{Z}_{\mathfrak{M}_\pm^{[1]}, \gamma}^*$  and  $Z_{\mathfrak{M}_\pm^{[1]}}^* := \|\mathbb{G}_n^{U*}\|_{\mathfrak{M}^{[1]}}$  satisfies the deviation bound: when  $n$  is sufficiently large,  $\forall \gamma \in (0, 1)$ ,

$$\Pr \left[ \left| Z_{\mathfrak{M}_\pm^{[1]}}^* - \tilde{Z}_{\mathfrak{M}_\pm^{[1]}, \gamma}^* \right| > C_1 \left( \frac{\log(n)^{2/3}}{\gamma^{1/3} (nh^3)^{1/6}} + \frac{\log(n)^{3/4}}{\gamma (nh^3)^{1/4}} \right) \right] \leq C_2 (\gamma + n^{-1})$$

and by Markov's inequality,

$$\Pr \left[ \Pr_{|W_1^n} \left[ \left| Z_{\mathfrak{M}_\pm^{[1]}}^* - \tilde{Z}_{\mathfrak{M}_\pm^{[1]}, \gamma}^* \right| > C_1 \left( \frac{\log(n)^{2/3}}{\gamma^{1/3} (nh^3)^{1/6}} + \frac{\log(n)^{3/4}}{\gamma (nh^3)^{1/4}} \right) \right] > \sqrt{C_2 (\gamma + n^{-1})} \right] \leq \sqrt{C_2 (\gamma + n^{-1})}.$$

By this result and (S51), when  $n$  is sufficiently large,  $\forall \gamma \in (0, 1)$ ,

$$\begin{aligned} \Pr \left[ \Pr_{|W_1^n} \left[ \left\| S^*(\cdot|x) \right\|_{I_x} - \tilde{Z}_{\mathfrak{M}_\pm^{[1]}, \gamma}^* > C_1 \left( \frac{\log(n)^{2/3}}{\gamma^{1/3} (nh^3)^{1/6}} + \frac{\log(n)^{3/4}}{\gamma (nh^3)^{1/4}} + \sqrt{\log(n)h} \right) \right] > \right. \\ \left. C_2 \left( \sqrt{\gamma} + \left( \frac{\log(n)}{nh^3} \right)^{1/4} \right) \right] \leq C_3 \left( \sqrt{\gamma} + \sqrt{\frac{\log(n)}{nh^3}} \right). \end{aligned}$$

Then, since  $\tilde{Z}_{\mathfrak{M}_{\pm}^{[1]}, \gamma}^*$  is independent of the data and  $\tilde{Z}_{\mathfrak{M}_{\pm}^{[1]}, \gamma}^* =_d \|G^U\|_{\mathfrak{M}^{[1]}}$ , by the above deviation bound and Chernozhukov et al. (2016, Lemma 2.1), with probability greater than  $1 - C_3 \left( \sqrt{\gamma} + \sqrt{\log(n)/(nh^3)} \right)$ ,

$$\sup_{t \in \mathbb{R}} |\Pr_{|W_1^n} [\|S^*(\cdot|x)\|_{I_x} \leq t] - \Pr [\|G^U\|_{\mathfrak{M}^{[1]}} \leq t]| \leq \sup_{t \in \mathbb{R}} \Pr \left[ \left| \|G^U\|_{\mathfrak{M}^{[1]}} - t \right| \leq C_1 \left( \frac{\log(n)^{2/3}}{\gamma^{1/3} (nh^3)^{1/6}} + \frac{\log(n)^{3/4}}{\gamma (nh^3)^{1/4}} + \sqrt{\log(n)h} \right) \right] + C_2 \left( \sqrt{\gamma} + \left( \frac{\log(n)}{nh^3} \right)^{1/4} \right).$$

By (48) and optimally choosing  $\gamma = \log(n)^{5/6} / (nh^3)^{1/6}$  (which balances  $\sqrt{\gamma}$  and  $\log(n)^{5/4} / (\gamma n^{1/4} h^{3/4})$ ), we have (34). By repeating the arguments used to show (52), we have  $|\Pr [\|S(\cdot|x)\|_{I_x} \leq s_{1-\alpha}^*] - (1-\alpha)| \leq C_1 \kappa_0 + C_2 \kappa_2^* + C_3 \kappa_3^*$ . The first conclusion follows.

The second conclusion follows from the second part of Lemma S3 and similar arguments.  $\blacksquare$

## S4 Proof of Theorem 3

**Proof of Theorem 3.** It follows from arguments used in previous proofs (see the proofs of Lemmas 2 and 3) that

$$\frac{1}{n} \sum_{i=1}^n \frac{1}{h} M \left( \frac{\hat{\Delta}_i - v}{h} \right)^2 \mathbb{1}(X_i = x) - \mathbb{E} \left[ \frac{1}{h} M \left( \frac{\Delta - v}{h} \right)^2 \mathbb{1}(X_i = x) \right] = O_p^* \left( \sqrt{\frac{\log(n)}{nh}}, \sqrt{\frac{\log(n)}{nh^3}} \right).$$

Therefore,  $\left\| \hat{\mathbb{V}}_{\Delta X}^\dagger(\cdot, x) - \mathbb{V}_{\Delta X}^\dagger(\cdot, x) \right\|_{I_x} = O_p^* \left( \sqrt{\log(n)/(nh)}, \sqrt{\log(n)/(nh^3)} \right)$ .

Denote

$$\begin{aligned} \tilde{\mathbb{V}}_{\Delta X}^\dagger(v, x) &:= \frac{1}{n_{(3)}} \sum_{(i,j,k)} \frac{1}{h^3} M' \left( \frac{\hat{\Delta}_j - v}{h} \right) q_x(W_j, W_i) M' \left( \frac{\hat{\Delta}_k - v}{h} \right) q_x(W_k, W_i) \mathbb{1}(X_i = x) \\ \bar{\mathbb{V}}_{\Delta X}^\dagger(v, x) &:= \frac{1}{n_{(3)}} \sum_{(i,j,k)} \frac{1}{h^3} M' \left( \frac{\Delta_j - v}{h} \right) q_x(W_j, W_i) M' \left( \frac{\Delta_k - v}{h} \right) q_x(W_k, W_i) \mathbb{1}(X_i = x). \end{aligned}$$

First,

$$\begin{aligned} \hat{\mathbb{V}}_{\Delta X}^\dagger(v, x) - \tilde{\mathbb{V}}_{\Delta X}^\dagger(v, x) &= \frac{2}{n_{(3)}} \sum_{(i,j,k)} \frac{1}{h^3} M' \left( \frac{\hat{\Delta}_j - v}{h} \right) (\hat{q}_x(W_j, W_i) - q_x(W_j, W_i)) M' \left( \frac{\hat{\Delta}_k - v}{h} \right) q_x(W_k, W_i) \mathbb{1}(X_i = x) \\ &+ \frac{1}{n_{(3)}} \sum_{(i,j,k)} \frac{1}{h^3} M' \left( \frac{\hat{\Delta}_j - v}{h} \right) (\hat{q}_x(W_j, W_i) - q_x(W_j, W_i)) M' \left( \frac{\hat{\Delta}_k - v}{h} \right) (\hat{q}_x(W_k, W_i) - q_x(W_k, W_i)) \mathbb{1}(X_i = x). \end{aligned} \tag{S52}$$

Then, by (S35),

$$\begin{aligned} \frac{1}{n_{(3)}} \sum_{(i,j,k)} \frac{1}{h^3} M' \left( \frac{\hat{\Delta}_j - v}{h} \right) (\hat{q}_{dx}(W_j, W_i) - q_{dx}(W_j, W_i)) M' \left( \frac{\hat{\Delta}_k - v}{h} \right) q_x(W_k, W_i) \mathbb{1}(X_i = x) = \\ T_1^\dagger(v) + T_2^\dagger(v) + T_3^\dagger(v) + T_4^\dagger(v), \end{aligned}$$

where

$$\begin{aligned}
T_1^\dagger(v) &:= \frac{1}{n_{(3)}} \sum_{(i,j,k)} \frac{1}{h^3} M' \left( \frac{\hat{\Delta}_j - v}{h} \right) \mathbb{1}(D_j = d', X_j = x) \mathbb{1}(D_i = d) \\
&\quad \times \frac{\left\{ \mathbb{1}(Y_i \leq \hat{\phi}_{dx}(Y_j)) - \mathbb{1}(Y_i \leq \phi_{dx}(Y_j)) \right\}}{\zeta_{dx}(\phi_{dx}(Y_j))} M' \left( \frac{\hat{\Delta}_k - v}{h} \right) q_x(W_k, W_i) \mathbb{1}(X_i = x) \\
T_2^\dagger(v) &:= \frac{1}{n_{(3)}} \sum_{(i,j,k)} \frac{1}{h^3} M' \left( \frac{\hat{\Delta}_j - v}{h} \right) \mathbb{1}(D_j = d', X_j = x) \\
&\quad \times \frac{\hat{R}_{d'x}(Y_j) - R_{d'x}(Y_j)}{\zeta_{dx}(\phi_{dx}(Y_j))} M' \left( \frac{\hat{\Delta}_k - v}{h} \right) q_x(W_k, W_i) \mathbb{1}(X_i = x) \\
T_3^\dagger(v) &:= \frac{1}{n_{(3)}} \sum_{(i,j,k)} \frac{1}{h^3} M' \left( \frac{\hat{\Delta}_j - v}{h} \right) \mathbb{1}(D_j = d', X_j = x) \\
&\quad \times \frac{\hat{\varphi}_{dx}(W_j, W_i) \left\{ \hat{\zeta}_{dx}(\hat{\phi}_{dx}(Y_j)) - \zeta_{dx}(\phi_{dx}(Y_j)) \right\}}{\zeta_{dx}(\phi_{dx}(Y_j))^2} M' \left( \frac{\hat{\Delta}_k - v}{h} \right) q_x(W_k, W_i) \mathbb{1}(X_i = x) \\
T_4^\dagger(v) &:= \frac{1}{n_{(3)}} \sum_{(i,j,k)} \frac{1}{h^3} M' \left( \frac{\hat{\Delta}_j - v}{h} \right) \mathbb{1}(D_j = d', X_j = x) \\
&\quad \times \frac{\hat{\varphi}_{dx}(W_j, W_i) \left\{ \hat{\zeta}_{dx}(\hat{\phi}_{dx}(Y_j)) - \zeta_{dx}(\phi_{dx}(Y_j)) \right\}^2}{\hat{\zeta}_{dx}(\hat{\phi}_{dx}(Y_j)) \zeta_{dx}(\phi_{dx}(Y_j))^2} M' \left( \frac{\hat{\Delta}_k - v}{h} \right) q_x(W_k, W_i) \mathbb{1}(X_i = x).
\end{aligned}$$

Denote  $\underline{\zeta}_{dx} := \inf_{y \in I_{dx}} |\zeta_{dx}(y)|$ . In view of (S12), when  $n$  is sufficiently large, with probability at least  $1 - C_2 n^{-1}$ ,

$$\begin{aligned}
|T_1^\dagger(v)| &\lesssim h^{-1} \underline{\zeta}_{dx}^{-2} \left\{ \bar{N}_x(v) + (nh)^{-1} \right\}^2 \max_{k=1, \dots, n} \left\{ N_k(v) \mathbb{1}(D_k = d', X_k = x) \right. \\
&\quad \left. \times \frac{1}{n} \sum_{i=1}^n \left| \mathbb{1}(Y_i \leq \hat{\phi}_{dx}(Y_k)) - \mathbb{1}(Y_i \leq \phi_{dx}(Y_k)) \right| \mathbb{1}(D_i = d, X_i = x) \right\}.
\end{aligned}$$

Now by this result, the fact that

$$\sup_{y \in I_{d'x}} \left| \frac{1}{n} \sum_{i=1}^n \left| \mathbb{1}(Y_i \leq \hat{\phi}_{dx}(y)) - \mathbb{1}(Y_i \leq \phi_{dx}(y)) \right| \mathbb{1}(D_i = d, X_i = x) \right| = O_p^* \left( \sqrt{\frac{\log(n)}{n}} \right)$$

and  $\|\bar{N}_x\|_{I_x} = O_p^*(1)$ ,  $\|T_1^\dagger\|_{I_x} = O_p^* \left( \sqrt{\log(n)/(nh^2)} \right)$ . Similarly, when  $n$  is sufficiently large, with probability at least  $1 - C_2 n^{-1}$ ,

$$\begin{aligned}
|T_2^\dagger(v)| &\lesssim h^{-1} \underline{\zeta}_{dx}^{-2} \left\{ \bar{N}_x(v) + (nh)^{-1} \right\}^2 \max_{k=1, \dots, n} \left\{ N_k(v) \mathbb{1}(D_k = d', X_k = x) \left| \hat{R}_{d'x}(Y_k) - R_{d'x}(Y_k) \right| \right\} \\
&= O_p^* \left( \sqrt{\frac{\log(n)}{nh^2}} \right),
\end{aligned}$$

uniformly in  $v \in I_x$ , where the equality follows from  $\|\bar{N}_x\|_{I_x} = O_p^*(1)$  and Lemma 4. Then, by  $\|\bar{N}_x\|_{I_x} = O_p^*(1)$

and (S36),

$$\begin{aligned} |T_3^\dagger(v)| &\lesssim h^{-1} \zeta_{dx}^{-2} \left\{ \bar{N}_x(v) + (nh)^{-1} \right\}^2 \max_{k=1, \dots, n} \left\{ N_k(v) \mathbb{1}(D_k = d', X_k = x) \left| \widehat{\zeta}_{dx}(\widehat{\phi}_{dx}(Y_k)) - \zeta_{dx}(\phi_{dx}(Y_k)) \right| \right\} \\ &= O_p^* \left( \sqrt{\frac{\log(n)}{nh^2 h_g}} + \frac{h_g^2}{h} \right), \end{aligned}$$

uniformly in  $v \in I_x$ . Similarly, since  $\inf_{y \in I_{d'x}} |\widehat{\zeta}_{dx}(\widehat{\phi}_{dx}(y))| > \inf_{y \in I_{d'x}} |\zeta_{dx}(\phi_{dx}(y))|/2$  with probability greater than  $1 - C_2 n^{-1}$  when  $n$  is sufficiently large,  $\|T_4^\dagger\|_{I_x} = O_p^* \left( \left( \sqrt{\log(n)/(nh_g)} + h_g^2 \right)^2 / h \right)$ . By tedious algebra, (S35), Lemma 4 and (S37),

$$\begin{aligned} &\frac{1}{n_{(3)}} \sum_{(i,j,k)} \frac{1}{h^3} M' \left( \frac{\widehat{\Delta}_j - v}{h} \right) (\widehat{q}_{dx}(W_j, W_i) - q_{dx}(W_j, W_i)) M' \left( \frac{\widehat{\Delta}_k - v}{h} \right) \\ &\quad \times (\widehat{q}_{dx}(W_k, W_i) - q_{dx}(W_k, W_i)) \mathbb{1}(X_i = x) = \\ &\quad \frac{1}{n_{(3)}} \sum_{(i,j,k)} \frac{1}{h^3} M' \left( \frac{\widehat{\Delta}_j - v}{h} \right) \mathbb{1}(D_j = d', X_j = x) \frac{\mathbb{1}(Y_i \leq \widehat{\phi}_{dx}(Y_j)) - \mathbb{1}(Y_i \leq \phi_{dx}(Y_j))}{\zeta_{dx}(\phi_{dx}(Y_j))} \\ &\quad \times M' \left( \frac{\widehat{\Delta}_k - v}{h} \right) \mathbb{1}(D_k = d', X_k = x) \frac{\mathbb{1}(Y_i \leq \widehat{\phi}_{dx}(Y_k)) - \mathbb{1}(Y_i \leq \phi_{dx}(Y_k))}{\zeta_{dx}(\phi_{dx}(Y_k))} \mathbb{1}(D_i = d, X_i = x) \\ &\quad + O_p^* \left( \sqrt{\frac{\log(n)}{nh^2}} \left( \sqrt{\frac{\log(n)}{nh_g}} + h_g^2 \right) \right) = O_p^* \left( \sqrt{\frac{\log(n)}{nh^2}} \right), \end{aligned}$$

uniformly in  $v \in I_x$ . Then, by these results and (S52),  $\|\widehat{V}_{\Delta X}^\dagger(\cdot, x) - \widetilde{V}_{\Delta X}^\dagger(\cdot, x)\|_{I_x} = O_p^* \left( \sqrt{\log(n)/(nh^2 h_g)} + h_g^2/h \right)$ .

Next,

$$\begin{aligned} \widetilde{V}_{\Delta X}^\dagger(v, x) - \bar{V}_{\Delta X}^\dagger(v, x) &= \\ &\frac{2}{n_{(3)}} \sum_{(i,j,k)} \frac{1}{h^3} \left\{ M' \left( \frac{\widehat{\Delta}_j - v}{h} \right) - M' \left( \frac{\Delta_j - v}{h} \right) \right\} q_x(W_j, W_i) M' \left( \frac{\Delta_k - v}{h} \right) q_x(W_k, W_i) \mathbb{1}(X_i = x) \\ &\quad + \frac{1}{n_{(3)}} \sum_{(i,j,k)} \frac{1}{h^3} \left\{ M' \left( \frac{\widehat{\Delta}_j - v}{h} \right) - M' \left( \frac{\Delta_j - v}{h} \right) \right\} q_x(W_j, W_i) \\ &\quad \times \left\{ M' \left( \frac{\widehat{\Delta}_k - v}{h} \right) - M' \left( \frac{\Delta_k - v}{h} \right) \right\} q_x(W_k, W_i) \mathbb{1}(X_i = x). \quad (\text{S53}) \end{aligned}$$

By triangle inequality, Taylor expansion, (S12) and  $\|\bar{N}_x\|_{I_x} = O_p^*(1)$ , the second term on the right hand side of (S53) is  $O_p^*(\log(n)/(nh^3))$ , uniformly in  $v \in I_x$ . By Taylor expansion, the first term can be written as

$$\begin{aligned} &\frac{2}{n_{(3)}} \sum_{(i,j,k)} \frac{1}{h^4} M'' \left( \frac{\Delta_j - v}{h} \right) (\widehat{\Delta}_j - \Delta_j) q_x(W_j, W_i) M' \left( \frac{\Delta_k - v}{h} \right) q_x(W_k, W_i) \mathbb{1}(X_i = x) \\ &\quad + \frac{1}{n_{(3)}} \sum_{(i,j,k)} \frac{1}{h^5} M^{(3)} \left( \frac{\Delta_j - v}{h} \right) (\widehat{\Delta}_j - \Delta_j)^2 q_x(W_j, W_i) M' \left( \frac{\Delta_k - v}{h} \right) q_x(W_k, W_i) \mathbb{1}(X_i = x) \\ &\quad =: 2 \cdot T_5^\dagger(v) + T_6^\dagger(v), \end{aligned}$$

where  $\hat{\Delta}_j$  is the mean value that lies between  $\hat{\Delta}_j$  and  $\Delta_j$ . Clearly,  $\|T_6^\dagger\|_{I_x} = O_p^*(\log(n)/(nh^3))$  and by Lemma 1 and  $\|\bar{N}_x\|_{I_x} = O_p^*(1)$ ,

$$T_5^\dagger(v) = \frac{1}{n^{(4)}} \sum_{(i,j,k,m)} \frac{1}{h^4} M''\left(\frac{\Delta_j - v}{h}\right) q_x(W_j, W_m) \pi_m q_x(W_j, W_i) M'\left(\frac{\Delta_k - v}{h}\right) q_x(W_k, W_i) \mathbb{1}(X_i = x) \\ + O_p^*\left(\left(\frac{\log(n)}{n}\right)^{3/4} h^{-2}\right)$$

and therefore,

$$T_5^\dagger(v) = \frac{1}{n^{(4)}} \sum_{(i,j,k,m)} \frac{1}{h^4} M''\left(\frac{\Delta_x(\epsilon_j) - v}{h}\right) \varpi_x(U_j) \{ \mathbb{1}(\epsilon_m \leq \epsilon_j) - F_{\epsilon|X}(\epsilon_j | x) \} \pi_m \\ \times \varpi_x(U_j) \{ \mathbb{1}(\epsilon_i \leq \epsilon_j) - F_{\epsilon|X}(\epsilon_j | x) \} M'\left(\frac{\Delta_x(\epsilon_k) - v}{h}\right) \varpi_x(U_k) \\ \times \{ \mathbb{1}(\epsilon_i \leq \epsilon_k) - F_{\epsilon|X}(\epsilon_k | x) \} \mathbb{1}(X_i = x) + O_p^*\left(\left(\frac{\log(n)}{n}\right)^{3/4} h^{-2}\right) \\ =: \frac{1}{n^{(4)}} \sum_{(i,j,k,m)} \mathcal{K}_x(U_i, U_j, U_k, U_m; v) + O_p^*\left(\left(\frac{\log(n)}{n}\right)^{3/4} h^{-2}\right),$$

where the leading term is written as a U-statistic. Let

$$\check{\mathcal{K}}_x(U_i, U_j, U_k, U_m; v) := \frac{1}{4!} \sum_{(i',j',k',m') \in \text{perm}\{i,j,k,m\}} \mathcal{K}_x(U_{i'}, U_{j'}, U_{k'}, U_{m'}; v) \quad (\text{S54})$$

denote the symmetrization of the kernel and then,

$$T_5^\dagger(v) = \frac{1}{n^{(4)}} \sum_{(i,j,k,m)} \check{\mathcal{K}}_x(U_i, U_j, U_k, U_m; v) + O_p^*\left(\left(\frac{\log(n)}{n}\right)^{3/4} h^{-2}\right). \quad (\text{S55})$$

Denote  $\check{\mathcal{K}}_x^{(1)}(u; v) := \mathbb{E}[\check{\mathcal{K}}_x(u, U_1, U_2, U_3; v)]$  and  $\check{\mathcal{K}}_x^{(2)}(u_1, u_2; v) := \mathbb{E}[\check{\mathcal{K}}_x(u_1, u_2, U_1, U_2; v)]$ . It is easy to see that  $\mathbb{E}[\check{\mathcal{K}}_x(U_1, U_2, U_3, U_4; v)] = 0, \forall v \in I_x$ . Denote  $\mathfrak{K} := \{\check{\mathcal{K}}_x(\cdot; v) : v \in I_x\}$ ,  $\mathfrak{K}^{(1)} := \{\check{\mathcal{K}}_x^{(1)}(\cdot; v) : v \in I_x\}$  and  $\mathfrak{K}^{(2)} := \{\check{\mathcal{K}}_x^{(2)}(\cdot; v) : v \in I_x\}$ . By similar arguments used in the proof of Lemma 3,  $\mathfrak{K}$  is uniformly VC-type with respect to a constant envelope  $F_{\mathfrak{K}} \propto h^{-4}$ . By Lemma A.3 of CK,  $\mathfrak{K}^{(1)}$  and  $\mathfrak{K}^{(2)}$  are also uniformly VC-type with respect to constant envelopes  $F_{\mathfrak{K}^{(1)}} = F_{\mathfrak{K}^{(2)}} = F_{\mathfrak{K}}$ .

Since  $\epsilon$  is independent of  $Z$  conditionally on  $X$ ,  $\mathbb{E}[\check{\mathcal{K}}_x^{(1)}(U; v)^2] = \mathbb{E}[(\mathbb{E}[\mathcal{K}_x(U_1, U_2, U_3, U_4; v) | U_4])^2]$ . Therefore,

$$\mathbb{E}[\check{\mathcal{K}}_x^{(1)}(U; v)^2] = \mathbb{E}\left[\frac{1}{h^4} \left\{ \int_{\epsilon_x}^{\bar{\epsilon}_x} \int_{\epsilon_x}^{\bar{\epsilon}_x} \frac{1}{h^2} M''\left(\frac{\Delta_x(e) - v}{h}\right) \varrho_x(e) \{ \mathbb{1}(\epsilon \leq e) - F_{\epsilon|X}(e | x) \} \right. \right. \\ \left. \left. \times \{ F_{\epsilon|X}(e \wedge e' | x) - F_{\epsilon|X}(e | x) F_{\epsilon|X}(e' | x) \} M'\left(\frac{\Delta_x(e') - v}{h}\right) \rho_x(e') \mathrm{d}e' \mathrm{d}e \right\}^2 \mid X = x \right] (p_{1x}^{-1} + p_{0x}^{-1}), \quad (\text{S56})$$

where  $\varrho_x(e) := f_{\epsilon DX}(e, 0, x) / \zeta_{1x}(g(1, x, e))^2 + f_{\epsilon DX}(e, 1, x) / \zeta_{0x}(g(0, x, e))^2$ . By the  $c_r$  inequality,

$$\begin{aligned} \mathbb{E} \left[ \left\{ \int_{\underline{\epsilon}_x}^{\bar{\epsilon}_x} \int_{\underline{\epsilon}_x}^{\bar{\epsilon}_x} \frac{1}{h^2} M'' \left( \frac{\Delta_x(e) - v}{h} \right) \varrho_x(e) \{ \mathbb{1}(\epsilon \leq e) - F_{\epsilon|X}(e|x) \} \right. \right. \\ \left. \times \{ F_{\epsilon|X}(e \wedge e' | x) - F_{\epsilon|X}(e|x) F_{\epsilon|X}(e' | x) \} \frac{1}{h^2} M' \left( \frac{\Delta_x(e') - v}{h} \right) \rho_x(e') \mathrm{d}e' \mathrm{d}e \right\}^2 \mid X = x \right] \leq \\ \sum_{k=1}^m \sum_{j=1}^m \mathbb{E} \left[ \left\{ \int_{\ell_{x,k-1}}^{\ell_{x,k}} \frac{1}{h^2} M'' \left( \frac{\Delta_x(e) - v}{h} \right) \varrho_x(e) \mathbb{1}(\epsilon \leq e) \vartheta_{x,j}(e; v) \mathrm{d}e \right\}^2 \mid X = x \right], \quad (\text{S57}) \end{aligned}$$

where

$$\vartheta_{x,j}(e; v) := \int_{\ell_{x,j-1}}^{\ell_{x,j}} \frac{1}{h^2} \{ F_{\epsilon|X}(e \wedge e' | x) - F_{\epsilon|X}(e|x) F_{\epsilon|X}(e' | x) \} M' \left( \frac{\Delta_x(e') - v}{h} \right) \rho_x(e') \mathrm{d}e'.$$

If  $k < j$ ,

$$\begin{aligned} \mathbb{E} \left[ \left\{ \int_{\ell_{x,k-1}}^{\ell_{x,k}} \frac{1}{h^2} M'' \left( \frac{\Delta_x(e) - v}{h} \right) \varrho_x(e) \mathbb{1}(\epsilon \leq e) \vartheta_{x,j}(e; v) \mathrm{d}e \right\}^2 \mid X = x \right] = \\ \mathbb{E} \left[ \left\{ \int_{\ell_{x,k-1}}^{\ell_{x,k}} \frac{1}{h^2} M'' \left( \frac{\Delta_x(e) - v}{h} \right) \varrho_x(e) \mathbb{1}(\epsilon \leq e) F_{\epsilon|X}(e|x) \mathrm{d}e \right\}^2 \mid X = x \right] \\ \times \left\{ \int_{\ell_{x,j-1}}^{\ell_{x,j}} \{ 1 - F_{\epsilon|X}(e' | x) \} \frac{1}{h^2} M' \left( \frac{\Delta_x(e') - v}{h} \right) \rho_x(e') \mathrm{d}e' \right\}^2. \quad (\text{S58}) \end{aligned}$$

By standard change of variables arguments,

$$\int_{\ell_{x,j-1}}^{\ell_{x,j}} \{ 1 - F_{\epsilon|X}(e' | x) \} \frac{1}{h^2} M' \left( \frac{\Delta_x(e') - v}{h} \right) \rho_x(e') \mathrm{d}e' = (\psi'_{x,j}(v) - \chi'_{x,j}(v)) + o(1) \quad (\text{S59})$$

and by similar arguments used to show (S30),

$$\begin{aligned} \mathbb{E} \left[ \left\{ \int_{\ell_{x,k-1}}^{\ell_{x,k}} \frac{1}{h^2} M'' \left( \frac{\Delta_x(e) - v}{h} \right) \varrho_x(e) \mathbb{1}(\epsilon \leq e) F_{\epsilon|X}(e|x) \mathrm{d}e \right\}^2 \mid X = x \right] = \\ h^{-4} \int_{\ell_{x,k-1}}^{\ell_{x,k}} \int_{\ell_{x,k-1}}^{\ell_{x,k}} M'' \left( \frac{\Delta_x(e) - v}{h} \right) M'' \left( \frac{\Delta_x(e') - v}{h} \right) F_{\epsilon|X}(e \wedge e' | x) F_{\epsilon|X}(e|x) \varrho_x(e) F_{\epsilon|X}(e' | x) \varrho_x(e') \mathrm{d}e \mathrm{d}e' \\ = O(h^{-1}), \end{aligned}$$

uniformly in  $v \in I_x$ . It follows from this result, (S58) and (S59) that

$$\mathbb{E} \left[ \left\{ \int_{\ell_{x,k-1}}^{\ell_{x,k}} \frac{1}{h^2} M'' \left( \frac{\Delta_x(e) - v}{h} \right) \varrho_x(e) \mathbb{1}(\epsilon \leq e) \vartheta_{x,j}(e; v) \mathrm{d}e \right\}^2 \mid X = x \right] = O(h^{-1}),$$

uniformly in  $v \in I_x$ . A similar result holds when  $k > j$ . If  $k = j$ , by change of variables and integration by parts,

for  $e \in (\iota_{x,j-1}, \iota_{x,j})$ ,

$$\begin{aligned}
\vartheta_{x,j}(e; v) &= F_{\epsilon|X}(e|x) \left\{ \int_e^{\iota_{x,j}} (1 - F_{\epsilon|X}(e'|x)) \frac{1}{h^2} M' \left( \frac{\Delta_x(e') - v}{h} \right) \rho_x(e') de' \right\} \\
&\quad + (1 - F_{\epsilon|X}(e|x)) \left\{ \int_{\iota_{x,j-1}}^e F_{\epsilon|X}(e'|x) \frac{1}{h^2} M' \left( \frac{\Delta_x(e') - v}{h} \right) \rho_x(e') de' \right\} \\
&= -F_{\epsilon|X}(e|x) \int_{\frac{\Delta_x(e)-v}{h}}^{\frac{\Delta_x(\iota_{x,j})-v}{h}} M(y) \{ \psi'_{x,j}(hy+v) - \chi'_{x,j}(hy+v) \} dy \\
&\quad - (1 - F_{\epsilon|X}(e|x)) \int_{\frac{\Delta_x(\iota_{x,j-1})-v}{h}}^{\frac{\Delta_x(e)-v}{h}} M(y) \chi'_{x,j}(hy+v) dy.
\end{aligned} \tag{S60}$$

Then it follows that

$$\begin{aligned}
\mathbb{E} \left[ \left\{ \int_{\iota_{x,j-1}}^{\iota_{x,j}} \frac{1}{h^2} M'' \left( \frac{\Delta_x(e) - v}{h} \right) \varrho_x(e) \mathbb{1}(\epsilon \leq e) \vartheta_{x,j}(e; v) de \right\}^2 \mid X = x \right] &= \\
h^{-2} \int_{\frac{\Delta_x(\iota_{x,j-1})-v}{h}}^{\frac{\Delta_x(\iota_{x,j})-v}{h}} \int_{\frac{\Delta_x(\iota_{x,j-1})-v}{h}}^{\frac{\Delta_x(\iota_{x,j})-v}{h}} M''(u) M''(w) F_{\epsilon|X}(\Upsilon_{x,j}(hu+v) \wedge \Upsilon_{x,j}(hw+v) \mid x) \\
\times \psi_{x,j}(hu+v) \vartheta_j(\Upsilon_{x,j}(hu+v); v) \psi_{x,j}(hw+v) \vartheta_j(\Upsilon_{x,j}(hw+v); v) dudw &= O(h^{-2}),
\end{aligned}$$

uniformly in  $v \in I_x$ . Therefore,  $\sigma_{\mathfrak{R}(1)}^2 := \sup_{f \in \mathfrak{R}(1)} \mathbb{P}^U f^2 = O(h^{-2})$ . It follows from the  $c_r$  inequality, change of variables and tedious but straightforward calculations,

$$\begin{aligned}
\mathbb{E} [\hat{\mathcal{K}}_x^{(2)}(U_1, U_2; v)^2] &\lesssim \mathbb{E} [(\mathbb{E}[\mathcal{K}_x(U_1, U_2, U_3, U_4; v) \mid U_1, U_4])^2] + \mathbb{E} [(\mathbb{E}[\mathcal{K}_x(U_1, U_2, U_3, U_4; v) \mid U_2, U_4])^2] \\
&\quad + \mathbb{E} [(\mathbb{E}[\mathcal{K}_x(U_1, U_2, U_3, U_4; v) \mid U_3, U_4])^2] \\
&= O(h^{-5}),
\end{aligned}$$

uniformly in  $v \in I_x$ . Therefore,  $\sigma_{\mathfrak{R}(2)}^2 := \sup_{f \in \mathfrak{R}(2)} \mathbb{P}^{(2)} f^2 = O(h^{-5})$ . Denote  $Z_{\mathfrak{R}\pm} := \left\| \mathbb{U}_n^{(4)} \right\|_{\mathfrak{R}}$ . By the coupling theorem (Proposition 2.1 of CK with  $\mathcal{H} = \mathfrak{R}_{\pm}$ ,  $\bar{\sigma}_{\mathfrak{g}} = \sigma_{\mathfrak{R}(1)}$ ,  $\sigma_{\mathfrak{h}} = \sigma_{\mathfrak{R}(2)}$ ,  $b_{\mathfrak{g}} = b_{\mathfrak{h}} = F_{\mathfrak{R}}$  and  $q = \infty$ ), when  $n$  is sufficiently large,  $\forall \gamma \in (0, 1)$ , there exists a random variable  $\tilde{Z}_{\mathfrak{R}\pm, \gamma} =_d \|G^U\|_{\mathfrak{R}(1)}$  such that

$$\Pr \left[ \left| Z_{\mathfrak{R}\pm} - \tilde{Z}_{\mathfrak{R}\pm, \gamma} \right| > C_1 \left( \frac{\log(n)^{2/3}}{n^{1/6} h^2 \gamma^{1/3}} + \frac{\log(n)}{n^{1/2} h^4 \gamma} \right) \right] \leq C_2 (\gamma + n^{-1}).$$

By the Borell-Sudakov-Tsirelson inequality,  $\Pr \left[ \|G^U\|_{\mathfrak{R}(1)} > \mathbb{E} [\|G^U\|_{\mathfrak{R}(1)}] + \sqrt{2 \cdot \log(n)} \sigma_{\mathfrak{R}(1)} \right] \leq n^{-1}$ . By Dudley's entropy integral bound,  $\mathbb{E} [\|G^U\|_{\mathfrak{R}(1)}] \lesssim (\sigma_{\mathfrak{R}(1)} \vee n^{-1/2} \|F_{\mathfrak{R}(1)}\|_{\mathbb{P}^U, 2}) \sqrt{\log(n)}$ . Therefore,

$$\Pr \left[ Z_{\mathfrak{R}\pm} > C_1 \left( \frac{\log(n)^{2/3}}{n^{1/6} h^2 \gamma^{1/3}} + \frac{\log(n)}{n^{1/2} h^4 \gamma} + \sqrt{\frac{\log(n)}{h^2}} \right) \right] \leq C_2 (\gamma + n^{-1}).$$

Therefore, it follows that when  $n$  is sufficiently large,  $\forall \gamma \in (0, 1)$ ,

$$\Pr \left[ \left\| \tilde{\mathbf{V}}_{\Delta X}^{\dagger}(\cdot, x) - \bar{\mathbf{V}}_{\Delta X}^{\dagger}(\cdot, x) \right\|_{I_x} > C_1 \left( \frac{\log(n)^{2/3}}{n^{2/3} h^2 \gamma^{1/3}} + \frac{\log(n)}{n h^4 \gamma} + \sqrt{\frac{\log(n)}{n h^2}} \right) \right] \leq C_2 (\gamma + n^{-1}).$$

By (39), we can write

$$\begin{aligned}
\bar{V}_{\Delta X}^\dagger(v, x) &= \frac{1}{n_{(3)}} \sum_{(i,j,k)} \frac{1}{h^3} K' \left( \frac{\Delta_x(\epsilon_j) - v}{h} \right) \varpi_x(U_j) \{ \mathbb{1}(\epsilon_i \leq \epsilon_j) - F_{\epsilon|X}(\epsilon_j | x) \} \\
&\quad \times K' \left( \frac{\Delta_x(\epsilon_k) - v}{h} \right) \varpi_x(U_k) \{ \mathbb{1}(\epsilon_i \leq \epsilon_k) - F_{\epsilon|X}(\epsilon_k | x) \} \mathbb{1}(X_i = x) \\
&=: \frac{1}{n_{(3)}} \sum_{(i,j,k)} \mathcal{J}_x(U_i, U_j, U_k; v).
\end{aligned}$$

We write  $\bar{V}_{\Delta X}^\dagger(v, x) = n_{(3)}^{-1} \sum_{(i,j,k)} \mathring{\mathcal{J}}_x(U_i, U_j, U_k; v)$ , where  $\mathring{\mathcal{J}}_x$  denotes the symmetrization of  $\mathcal{J}_x$  (see (S54)). Note that  $\bar{V}_{\Delta X}(v, x) = \mathbb{E}[\mathring{\mathcal{J}}_x(U_1, U_2, U_3; v)]$ . Denote  $\mathring{\mathcal{J}}_x^{(1)}(u; v) := \mathbb{E}[\mathring{\mathcal{J}}_x(u, U_1, U_2; v)]$ ,  $\mathring{\mathcal{J}}_x^{(2)}(u_1, u_2; v) := \mathbb{E}[\mathring{\mathcal{J}}_x(u_1, u_2, U_1; v)]$ ,  $\mathfrak{J} := \{\mathring{\mathcal{J}}_x(\cdot; v) : v \in I_x\}$ ,  $\mathfrak{J}^{(1)} := \{\mathring{\mathcal{J}}_x^{(1)}(\cdot; v) : v \in I_x\}$  and  $\mathfrak{J}^{(2)} := \{\mathring{\mathcal{J}}_x^{(2)}(\cdot; v) : v \in I_x\}$ . By similar arguments used in the proof of Lemma 3,  $\mathfrak{J}$  is uniformly VC-type with respect to a constant envelope  $F_{\mathfrak{J}} \propto h^{-3}$ . By Lemma A.3 of CK,  $\mathfrak{J}^{(1)}$  and  $\mathfrak{J}^{(2)}$  are also uniformly VC-type with respect to constant envelopes  $F_{\mathfrak{J}^{(1)}} = F_{\mathfrak{J}^{(2)}} = F_{\mathfrak{J}}$ .

Denote  $f_{\epsilon X}(e, x) := f_{\epsilon|X}(e | x) p_x$ . Then we have

$$\begin{aligned}
\mathbb{E}[(\mathbb{E}[\mathcal{J}_x(U_1, U_2, U_3; v) | U_1])^2] &= \\
&\int_{\underline{\epsilon}_x}^{\bar{\epsilon}_x} \frac{1}{h^2} \left\{ \int_{\underline{\epsilon}_x}^{\bar{\epsilon}_x} \frac{1}{h} M' \left( \frac{\Delta_x(e) - v}{h} \right) \rho_x(e) \{ \mathbb{1}(e' \leq e) - F_{\epsilon|X}(e | x) \} de \right\}^4 f_{\epsilon X}(e', x) de' \lesssim \\
&\sum_{k=1}^m \sum_{j=1}^m \int_{\iota_{x,k-1}}^{\iota_{x,k}} \frac{1}{h^2} \left\{ \int_{\iota_{x,j-1}}^{\iota_{x,j}} \frac{1}{h} M' \left( \frac{\Delta_x(e) - v}{h} \right) \rho_x(e) \{ \mathbb{1}(e' \leq e) - F_{\epsilon|X}(e | x) \} de \right\}^4 f_{\epsilon X}(e', x) de', \quad (\text{S61})
\end{aligned}$$

$$\begin{aligned}
\mathbb{E}[(\mathbb{E}[\mathcal{J}_x(U_1, U_2, U_3; v) | U_3])^2] &= \left\{ \int_{\underline{\epsilon}_x}^{\bar{\epsilon}_x} \frac{1}{h^2} M' \left( \frac{\Delta_x(e) - v}{h} \right)^2 \varrho_x(e)^2 \right. \\
&\quad \times \left. \left( \int_{\underline{\epsilon}_x}^{\bar{\epsilon}_x} \frac{1}{h^2} M' \left( \frac{\Delta_x(e') - v}{h} \right) \rho_x(e') \{ F_{\epsilon|X}(e \wedge e' | x) - F_{\epsilon|X}(e | x) F_{\epsilon|X}(e' | x) \} de' \right)^2 de \right\} p_x^2 \lesssim \\
&\sum_{k=1}^m \sum_{j=1}^m \left\{ \int_{\iota_{x,k-1}}^{\iota_{x,k}} \frac{1}{h^2} M' \left( \frac{\Delta_x(e) - v}{h} \right)^2 \varrho_x(e)^2 \vartheta_j(e; v)^2 de \right\} p_x^2 \quad (\text{S62})
\end{aligned}$$

and  $\mathbb{E}[(\mathbb{E}[\mathcal{J}_x(U_1, U_2, U_3; v) | U_2])^2] = \mathbb{E}[(\mathbb{E}[\mathcal{J}_x(U_1, U_2, U_3; v) | U_3])^2]$ . If  $k < j$ , by (S59),

$$\int_{\iota_{x,k-1}}^{\iota_{x,k}} \frac{1}{h^2} \left\{ \int_{\iota_{x,j-1}}^{\iota_{x,j}} \frac{1}{h} M' \left( \frac{\Delta_x(e) - v}{h} \right) \rho_x(e) \{ \mathbb{1}(e' \leq e) - F_{\epsilon|X}(e | x) \} de \right\}^4 f_{\epsilon X}(e', x) de' = O(h^2),$$

uniformly in  $v \in I_x$ . A similar result holds if  $k > j$ . If  $k = j$ , since for  $e' \in (\iota_{x,j-1}, \iota_{x,j})$ , by integration by parts and change of variables,

$$\int_{\iota_{x,j-1}}^{\iota_{x,j}} \frac{1}{h} M' \left( \frac{\Delta_x(e) - v}{h} \right) \rho_x(e) \mathbb{1}(e' \leq e) de = -M \left( \frac{\Delta_x(e') - v}{h} \right) \psi_{x,j}(\Delta_x(e'))$$

$$-h \int_{\frac{\Delta_x(e')-v}{h}}^{\frac{\Delta_x(\iota_{x,j})-v}{h}} M(u) \psi_{x,j}(hu+v) du,$$

then we have

$$\int_{\iota_{x,j-1}}^{\iota_{x,j}} \frac{1}{h^2} \left\{ \int_{\iota_{x,j-1}}^{\iota_{x,j}} \frac{1}{h} M' \left( \frac{\Delta_x(e)-v}{h} \right) \rho_x(e) \{ \mathbb{1}(e' \leq e) - F_{\epsilon|X}(e|x) \} de \right\}^4 f_{\epsilon X}(e',x) de' = O(h^{-1}),$$

uniformly in  $v \in I_x$ . It follows from these calculations and (S61) that  $\mathbb{E} \left[ (\mathbb{E}[\mathcal{J}_x(U_1, U_2, U_3; v) | U_1])^2 \right] = O(h^{-1})$ . If  $k < j$ , by change of variables,

$$\begin{aligned} \int_{\iota_{x,k-1}}^{\iota_{x,k}} \frac{1}{h^2} M' \left( \frac{\Delta_x(e)-v}{h} \right)^2 \varrho_x(e)^2 \vartheta_{x,j}(e;v)^2 de &= \left\{ \int_{\iota_{x,k-1}}^{\iota_{x,k}} \frac{1}{h^2} M' \left( \frac{\Delta_x(e)-v}{h} \right)^2 \varrho_x(e)^2 F_{\epsilon|X}(e|x)^2 de \right\} \\ &\times \left\{ \int_{\iota_{x,j-1}}^{\iota_{x,j}} \{1 - F_{\epsilon|X}(e'|x)\} \frac{1}{h^2} K' \left( \frac{\Delta_x(e')-v}{h} \right) \rho_x(e') de' \right\}^2 = O(h^{-1}), \end{aligned}$$

uniformly in  $v \in I_x$ . If  $k = j$ , by (S60) and change of variables,

$$\int_{\iota_{x,j-1}}^{\iota_{x,j}} \frac{1}{h^2} M' \left( \frac{\Delta_x(e)-v}{h} \right)^2 \varrho_x(e)^2 \vartheta_{x,j}(e;v)^2 de = O(h^{-1}),$$

uniformly in  $v \in I_x$ . It follows from these calculations and (S62) that  $\mathbb{E} \left[ (\mathbb{E}[\mathcal{J}_x(U_1, U_2, U_3; v) | U_2])^2 \right] = \mathbb{E} \left[ (\mathbb{E}[\mathcal{J}_x(U_1, U_2, U_3; v) | U_3])^2 \right] = O(h^{-1})$ . Then, by the  $c_r$  inequality,

$$\begin{aligned} \mathbb{E} \left[ \mathring{\mathcal{J}}_x^{(1)}(U; v)^2 \right] &\leq \mathbb{E} \left[ (\mathbb{E}[\mathcal{J}_x(U_1, U_2, U_3; v) | U_1])^2 \right] + \mathbb{E} \left[ (\mathbb{E}[\mathcal{J}_x(U_1, U_2, U_3; v) | U_2])^2 \right] \\ &\quad + \mathbb{E} \left[ (\mathbb{E}[\mathcal{J}_x(U_1, U_2, U_3; v) | U_3])^2 \right] \\ &= O(h^{-1}), \end{aligned}$$

uniformly in  $v \in I_x$ . Therefore,  $\sigma_{\mathfrak{J}^{(1)}}^2 := \sup_{f \in \mathfrak{J}^{(1)}} \mathbb{P}^U f^2 = O(h^{-1})$ . It is easy to check that

$$\begin{aligned} \mathbb{E} \left[ \mathring{\mathcal{J}}_x^{(2)}(U_1, U_2; v)^2 \right] &\leq \mathbb{E} \left[ (\mathbb{E}[\mathcal{J}_x(U_1, U_2, U_3; v) | U_2, U_3])^2 \right] + \mathbb{E} \left[ (\mathbb{E}[\mathcal{J}_x(U_1, U_2, U_3; v) | U_1, U_3])^2 \right] \\ &\quad + \mathbb{E} \left[ (\mathbb{E}[\mathcal{J}_x(U_1, U_2, U_3; v) | U_1, U_2])^2 \right] \\ &= O(h^{-4}), \end{aligned}$$

uniformly in  $v \in I_x$ . Therefore,  $\sigma_{\mathfrak{J}^{(2)}}^2 := \sup_{f \in \mathfrak{J}^{(2)}} \mathbb{P}^{(2)} f^2 = O(h^{-4})$ . Denote  $Z_{\mathfrak{J}^\pm} := \left\| \mathbb{U}_n^{(3)} \right\|_{\mathfrak{J}}$ . By the coupling theorem (Proposition 2.1 of CK with  $\mathcal{H} = \mathfrak{J}_\pm$ ,  $\bar{\sigma}_{\mathfrak{g}} = \sigma_{\mathfrak{J}^{(1)}}$ ,  $\sigma_{\mathfrak{h}} = \sigma_{\mathfrak{J}^{(2)}}$ ,  $b_{\mathfrak{g}} = b_{\mathfrak{h}} = F_{\mathfrak{J}}$ ,  $q = \infty$  and  $\gamma = \sqrt{\log(n)/(nh^3)}$ ), when  $n$  is sufficiently large,  $\Pr \left[ \left| Z_{\mathfrak{J}^\pm} - \tilde{Z}_{\mathfrak{J}^\pm} \right| > C_1 \sqrt{\log(n)/h^3} \right] \leq C_2 \sqrt{\log(n)/(nh^3)}$ , where  $\tilde{Z}_{\mathfrak{J}^\pm} = d \left\| G^U \right\|_{\mathfrak{J}^{(1)}}$ . By the Borell-Sudakov-Tsirelson inequality,  $\Pr \left[ \left\| G^U \right\|_{\mathfrak{J}^{(1)}} > \mathbb{E} \left[ \left\| G^U \right\|_{\mathfrak{J}^{(1)}} \right] + \sqrt{2 \cdot \log(n)} \sigma_{\mathfrak{J}^{(1)}} \right] \leq n^{-1}$ . By Dudley's entropy integral bound,  $\mathbb{E} \left[ \left\| G^U \right\|_{\mathfrak{J}^{(1)}} \right] \lesssim \left( \sigma_{\mathfrak{J}^{(1)}} \vee n^{-1/2} \left\| F_{\mathfrak{J}^{(1)}} \right\|_{\mathbb{P}^{U,2}} \right) \sqrt{\log(n)}$ . It follows that  $\Pr \left[ Z_{\mathfrak{J}^\pm} > C_1 \sqrt{\log(n)/h^3} \right] \leq C_2 \sqrt{\log(n)/(nh^3)}$  and therefore, we have  $\left\| \bar{\mathbb{V}}_{\Delta X}^\dagger(\cdot, x) - \mathbb{V}_{\Delta X}^\dagger(\cdot, x) \right\|_{I_x} = O_p^* \left( \sqrt{\log(n)/(nh^3)}, \sqrt{\log(n)/(nh^3)} \right)$ , where  $\bar{\mathbb{V}}_{\Delta X}^\dagger(\cdot, x) = n_{(3)}^{-1} \sum_{(i,j,k)} \mathring{\mathcal{J}}_x(U_i, U_j, U_k; v)$  and  $\bar{\mathbb{V}}_{\Delta X}(v, x) = \mathbb{E} \left[ \mathring{\mathcal{J}}_x(U_1, U_2, U_3; v) \right]$ .

Table S1: Coverage rates for point-wise confidence intervals

| $v$ | $n$  | Methods | $\gamma_0 = -0.5, \gamma_1 = 0.5$ |       |       | $\gamma_0 = -0.4, \gamma_1 = 0.6$ |       |       |
|-----|------|---------|-----------------------------------|-------|-------|-----------------------------------|-------|-------|
|     |      |         | 0.90                              | 0.95  | 0.99  | 0.90                              | 0.95  | 0.99  |
| 1.6 | 2000 | PA      | 0.890                             | 0.933 | 0.981 | 0.878                             | 0.924 | 0.973 |
|     |      | PB      | 0.936                             | 0.975 | 0.996 | 0.943                             | 0.979 | 0.999 |
|     | 4000 | PA      | 0.901                             | 0.951 | 0.980 | 0.900                             | 0.946 | 0.978 |
|     |      | PB      | 0.916                             | 0.961 | 0.994 | 0.931                             | 0.970 | 0.995 |
|     | 6000 | PA      | 0.902                             | 0.951 | 0.980 | 0.907                             | 0.950 | 0.981 |
|     |      | PB      | 0.927                             | 0.974 | 0.994 | 0.944                             | 0.979 | 0.995 |
| 2.0 | 2000 | PA      | 0.900                             | 0.940 | 0.977 | 0.874                             | 0.914 | 0.954 |
|     |      | PB      | 0.935                             | 0.977 | 0.997 | 0.939                             | 0.982 | 0.997 |
|     | 4000 | PA      | 0.897                             | 0.945 | 0.984 | 0.895                             | 0.945 | 0.975 |
|     |      | PB      | 0.934                             | 0.975 | 0.996 | 0.950                             | 0.980 | 0.997 |
|     | 6000 | PA      | 0.900                             | 0.953 | 0.987 | 0.909                             | 0.949 | 0.988 |
|     |      | PB      | 0.928                             | 0.967 | 0.997 | 0.946                             | 0.972 | 0.999 |
| 2.4 | 2000 | PA      | 0.874                             | 0.915 | 0.950 | 0.832                             | 0.880 | 0.922 |
|     |      | PB      | 0.934                             | 0.972 | 0.991 | 0.940                             | 0.974 | 0.997 |
|     | 4000 | PA      | 0.887                             | 0.931 | 0.976 | 0.872                             | 0.925 | 0.962 |
|     |      | PB      | 0.944                             | 0.970 | 0.997 | 0.945                             | 0.978 | 0.998 |
|     | 6000 | PA      | 0.901                             | 0.948 | 0.986 | 0.901                             | 0.939 | 0.979 |
|     |      | PB      | 0.938                             | 0.969 | 0.999 | 0.945                             | 0.977 | 0.997 |

Since

$$\widehat{V}_{\Delta X}^{\dagger}(v, x) - V_{\Delta X}^{\dagger}(v, x) = \left( \widehat{V}_{\Delta X}^{\dagger}(v, x) - \widetilde{V}_{\Delta X}^{\dagger}(v, x) \right) + \left( \widetilde{V}_{\Delta X}^{\dagger}(v, x) - \overline{V}_{\Delta X}^{\dagger}(v, x) \right) + \left( \overline{V}_{\Delta X}^{\dagger}(v, x) - V_{\Delta X}^{\dagger}(v, x) \right),$$

it follows from previous results that  $\Pr \left[ \left\| \widehat{V}_{\Delta X}^{\dagger}(\cdot, x) - V_{\Delta X}^{\dagger}(\cdot, x) \right\|_{I_x} > C_1 \kappa_1^{\dagger} \right] \leq C_2 \kappa_2^{\dagger}$ , when  $n$  is sufficiently large. The conclusion follows from this result,  $\left\| \widehat{V}_{\Delta X}^{\dagger}(\cdot, x) - V_{\Delta X}^{\dagger}(\cdot, x) \right\|_{I_x} = O_p^* \left( \sqrt{\log(n)/(nh)}, \sqrt{\log(n)/(nh^3)} \right)$  and

$$\widehat{V}_{\Delta|X}(v | x) - V_{\Delta|X}(v | x) = \frac{\widehat{V}_{\Delta X}(v, x)}{p_x^2} \left( \frac{p_x^2}{\widehat{p}_x^2} - 1 \right) + \frac{1}{p_x^2} \left( \widehat{V}_{\Delta X}(v, x) - V_{\Delta X}(v, x) \right).$$

■

## S5 Additional Monte Carlo simulation results

Table S1 presents the coverage rates of two types of pointwise confidence intervals for the density  $f_{\Delta}(v)$  evaluated at 1.6, 2.0 and 2.4. The method “PA” corresponds to the plug-in approach using our new standard errors and standard normal critical values (see Remark 5). The method “PB” corresponds to the bootstrap percentile confidence interval. The number of Monte Carlo replications is 1,000 and the nominal probability coverages rates are 0.90, 0.95 and 0.99. As Table S1 shows, PA produces coverage rates that are very close to the nominal levels, especially when the sample size is large. On the other hand, PB, though circumvents the calculation of standard errors, exhibits certain degree of over-coverage.

## References

- Abadie, A. (2003). Semiparametric instrumental variable estimation of treatment response models. *Journal of Econometrics* 113(2).
- Angrist, J., V. Chernozhukov, and I. Fernández-Val (2006). Quantile Regression under Misspecification, with an Application to the U.S. Wage Structure. *Econometrica* 74(2), 539–563.
- Chernozhukov, V., D. Chetverikov, and K. Kato (2014). Gaussian approximation of suprema of empirical processes. *The Annals of Statistics* 42(4), 1564–1597.
- Chernozhukov, V., D. Chetverikov, and K. Kato (2016). Empirical and multiplier bootstraps for suprema of empirical processes of increasing complexity, and related gaussian couplings. *Stochastic Processes and their Applications* 126(12), 3632–3651.
- Giné, E. and R. Nickl (2016). *Mathematical foundations of infinite-dimensional statistical models*, Volume 40. Cambridge University Press.
- Kosorok, M. R. (2007). *Introduction to empirical processes and semiparametric inference*. Springer Science & Business Media.
